# Supplementary material for: Long ties accelerate noisy threshold-based contagions
Source: arXiv:1810.03579 source file (2023-08-20)
Supplement: Supplementary file 1 [file pnas-si-long.pdf]

# Supplementary Information for

## Long ties accelerate noisy threshold-based contagions

Dean Eckles, Elchanan Mossel, M. Amin Rahimian and Subhabrata Sen

E-mails:{eckles,elmos,rahimian,ssen90}@mit.edu

### This PDF file includes:

- Supplementary text
- Figs. S1 to S9
- Table S1
- References for SI reference citations

### Supporting Information Text

This Supplementary Information is organized in four sections that parallel the four parts of the Results section in the main text. Sections S2, S3, and S4 include the proofs for Theorems 1, 2 and 3 from the main text, as well as additional simulations. In Section S5, we expand on our study of empirical networks and present additional simulation results under various contagion models that deviate from those considered in the main text. These additional results support the robustness of our claims against modeling variations.

**Notation:** For convenience of the reader, we collect here some notation that will be used throughout in the subsequent discussion. For sequences of real numbers, we use the usual Bachman-Landau notation  $O(\cdot)$ ,  $o(\cdot)$  and  $\Theta(\cdot)$ . Further, for a sequence of non-negative real numbers  $\{a_n : n \geq 1\}$  and a sequence of random variables  $\{X_n : n \geq 1\}$ , we say that  $X_n = o(a_n)$  if  $X_n/a_n \xrightarrow{P} 0$  as  $n \rightarrow \infty$ . Similarly, we declare  $X_n = O(a_n)$  if there exists a universal constant  $C > 0$  such that  $\mathbb{P}(|X_n|/a_n \leq C) \rightarrow 1$  as  $n \rightarrow \infty$ . Finally, say that  $X_n = \Theta(a_n)$  if there exist universal constants  $0 < c < C < \infty$  such that  $\mathbb{P}(ca_n < X_n < Ca_n) \rightarrow 1$  as  $n \rightarrow \infty$ . For two random variables  $X, Y$ , we set  $X \preceq Y$  if  $X$  is stochastically dominated by  $Y$ . A sequence of events  $\{A_n\}$  occurs with high probability as  $n \rightarrow \infty$  (referred to as w.h.p.) if  $\mathbb{P}(A_n^c) \rightarrow 0$  as  $n \rightarrow \infty$ .

### S1. Adoption probabilities by the number of adopting peers in real data

We use a number of prior empirical studies to report on the relative rates of adoptions when there are  $k$  and  $k - 1$  adopting neighbors:  $p(k)/p(k - 1)$ , for integers  $k > 1$ . We find that the reported ratios are less than five, consistently, across a multitude of studies (Figure S1); thus, there is evidence against homogeneous deterministic thresholds for adoption.

Aral et al. (2009) in (1) delineate how much of the clustering in the observed patterns of adoptions can be explained by contagion as opposed to homophily. The adoption patterns demonstrate significant clustering in terms of both network location of the adopters as well as the time at which neighboring nodes become adopters. However, the correlated outcomes can be attributed to both contagion and homophily: On the one hand, the linked nodes influence each other in their decisions to adopt; and on the other hand, they simply have greater likelihoods of displaying correlated outcomes as a consequence of their similar attributes. Using a dynamic matched sample estimation framework\*, Aral et al. (2009) show that previous methods over-estimate peer influence in a study of the global instant messaging network of 27.4 million users, using data on the day-by-day adoption of a mobile service application called Yahoo Go mobile. In Fig. 3B (right inset) of (1), Aral et al. (2009) report the adoption ratios among the matched pairs versus the number of adopter friends. We have extracted and plotted these ratios in Figure S1.

In (2), Bakshy et al. (2012) present their results from a large-scale field experiment about sharing URLs on Facebook with 253 million subjects. The experiment randomizes whether or not individuals are exposed via Facebook to information about their friends' sharing behavior. The authors find that additional exposure has an increasing causal effect on the propensity to share. We extracted the probability of sharing versus the number of sharing friends

\*They consider four different treatment levels corresponding to having one, two, three, or four adopter friends and estimate the treatment probabilities at different levels as a function of observable and latent node characteristics using logistic regression. They use the estimated treatment probabilities to create a dynamic matched sample of treated and untreated nodes over time: Every treated node (having one or more friends who are adopters) is matched with an untreated node (having fewer number of adopter friends) whose likelihoods of being treated (propensity scores) are closest.

on the Facebook News Feed from Fig. 4(a) of (2). This is the observational association, as the experiment only randomizes exposure or non-exposure. We have plotted the ratio of probabilities for different values of  $k$  in Figure S1.

In a controlled study to test for effects of complex contagion in (3), Centola (2010) randomizes subjects between two network conditions: a clustered lattice consisting entirely of short ties, and a random regular graph with very few triangle (short ties). The node degrees in both conditions are fixed and the same. The author studies the spread of a health-related behavior (registering for a health forum website) in an online community in which users were informed about the activities of their assigned neighbors (“health buddies”) through email invitations to adopt the same behavior. The faster spread over the clustered lattice has been interpreted as evidence of complex contagion. In Figure S1, we have extracted the values reported in Figure 3 of (3), where up to three additional social signals significantly increases the probability of adoption.

Mønsted et al. (2017) in (4) present the results of a non-randomized field experiment conducted on the Twitter social network. They test the adoption of new hashtags using a network of Twitter bots (“botnet”) with a large number of followers. The large user base who follow multiple bots are exposed to coordinated interventions by the bots to test the effects of multiple exposures. They observe that their proposed model of complex contagion is a better fit to the observed adoption rates than an alternative simple contagion model. We have extracted the percentage of retweets versus the total number of unique exposures from Figure 3A of (4) and plotted the results in Figure S1.

In (5), Ugander et al. (2012) use e-mail invitations for joining Facebook to study the growth of Facebook’s user base. In a corpus of 54 million such email invitations, they analyze the probability of accepting an invitation as a function of the structure of the contact neighborhoods. They observe that adoption probabilities are better explained by the number of connected components in the contact neighborhoods; thus highlighting the effect of structural diversity in determining the conversion decisions. In Figure S1, we have plotted the ratios of the aggregate conversion rates for each neighborhood size. This data, provided by the authors, is presented in their Figure 1.

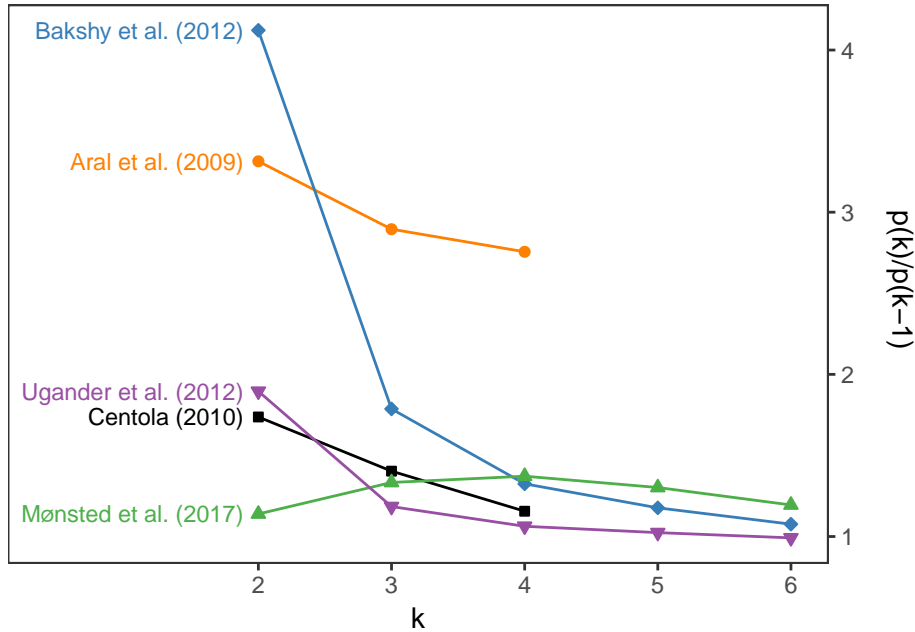

Fig. S1. Empirical adoption rate ratios

## S2. Spread of complex contagion over $\mathcal{C}_2$ union random graphs (Theorem 1)

In this section we provide the asymptotic rate of 2-complex contagion over  $\mathcal{C}_2 \cup \mathcal{G}_{n,c/n}$ , and compare it with  $\mathcal{C}_{2+c/2}$ . We conclude that the diffusion speed is faster in the rewired graph. Therefore, we emphasize the understanding that rewiring facilitates the spread of complex contagion as long as the required structure for total spread ( $\mathcal{C}_2$ ) is intact.

### A. Spreading time lower-bound for complex contagion.

**Theorem S2.1** (Upper-Bounding the number of infected nodes until  $t = o(n^{2/3})$ ). *Let  $I_t$  denote the number of infected nodes at time  $t$ . For  $t = o(n^{2/3})$ ,  $I_t = o(n^{2/3})$ .*

*Proof.* Let  $\mathcal{I}_t$  be the set of all infected nodes at time  $t$  and let  $\mathcal{B}_t$  denote the interval of length  $2t$  from the deterministic growth of the two neighboring initial seeds. Note that the vertices in  $\mathcal{B}_t$  are always infected due to two-complex contagion along  $\mathcal{C}_2$ ; hence,  $B_t = |\mathcal{B}_t| = 2t = T$ . We define  $\mathcal{I}_t^0 = \mathcal{B}_t$  and note that  $\mathcal{I}_t^0 \subset \mathcal{I}_t$ . However, other vertices might be infected due to complex contagion along the edges of  $\mathcal{G}_{n,c/n}$ . To control these secondary infections, we introduce an algorithm which proceeds in rounds. These rounds are indexed by  $\tau$  and they build up the infected set  $\{\mathcal{I}_t^\tau : \tau \geq 1\}$  by exposing new random edges connecting infected vertices, identified at the current round, to “healthy”-vertices. The analysis below tracks the growth of the infected set over iterations, and establishes that for  $t = o(n^{2/3})$ , the algorithm terminates after two rounds with high probability. Further, the additional infected vertices gained are  $o(n^{2/3})$  in number, and all isolated. Thus they do not give rise to secondary infections along  $\mathcal{C}_2$  via 2-complex contagion.

Let us introduce the sequential algorithm formally before we proceed further. For notational convenience, let  $\{\mathcal{S}_t^\tau : \tau \geq 1\}$  denote nodes with exactly one neighbor in  $\mathcal{I}_t^\tau$  and call them “susceptible” nodes. Further, let  $\mathcal{H}_t^\tau$  denote nodes that have no neighbors in  $\mathcal{I}_t^\tau$  and call them “healthy” nodes. Moreover, we denote the nodes that are added to the infected set at round  $\tau$  by  $\mathcal{A}_t^\tau = \mathcal{I}_t^\tau \setminus \mathcal{I}_t^{\tau-1}$ . Finally, for  $v \in [n]$  and  $C \subset [n]$ ,  $\mathcal{N}_C(v)$  will denote the number of neighbors of  $v$  in the set  $C$ .

**Algorithm: Edge-Revelation**

- Initialize:
  - $\mathcal{I}_t^{-1} = \emptyset$ ,  $\mathcal{I}_t^0 = \mathcal{B}_t$ ,  $\mathcal{A}_t^0 = \mathcal{B}_t$ ,  $\mathcal{S}_t^0 = \emptyset$ ,  $\mathcal{H}_t^0 = [n] \setminus (\mathcal{I}_t^0 \cup \mathcal{S}_t^0)$ .
- For  $\tau \geq 1$ , given  $(\mathcal{I}_t^{\tau-1}, \mathcal{A}_t^{\tau-1}, \mathcal{S}_t^{\tau-1}, \mathcal{H}_t^{\tau-1})$ :
  - Reveal all the long ties that are incident to  $\mathcal{A}_t^{\tau-1}$ .
  - Update the sets using the revealed edges:
    - \*  $\bar{\mathcal{S}}_t^\tau = \{v \in \mathcal{S}_t^{\tau-1} : \mathcal{N}_{\mathcal{I}_t^{\tau-1} \setminus \mathcal{I}_t^{\tau-2}}(v) \geq 1\}$ .  
These are the vertices that are susceptible at round  $\tau - 1$  and join the infected at round  $\tau$ .
    - \*  $\bar{\mathcal{H}}_t^\tau = \{v \in \mathcal{H}_t^{\tau-1} : \mathcal{N}_{\mathcal{I}_t^{\tau-1} \setminus \mathcal{I}_t^{\tau-2}}(v) \geq 2\}$ .  
These are the vertices that are healthy at round  $\tau - 1$  and join the infected at round  $\tau$ .
    - \*  $\hat{\mathcal{H}}_t^\tau = \{v \in \mathcal{H}_t^{\tau-1} : \mathcal{N}_{\mathcal{I}_t^{\tau-1}}(v) = 1\} = \{v \in \mathcal{H}_t^{\tau-1} : \mathcal{N}_{\mathcal{I}_t^{\tau-1} \setminus \mathcal{I}_t^{\tau-2}}(v) = 1\}$ .  
These are the healthy vertices at round  $\tau - 1$  that join the susceptible set at round  $\tau$ .
    - \*  $\mathcal{A}_t^\tau = \bar{\mathcal{S}}_t^\tau \cup \bar{\mathcal{H}}_t^\tau$ , these are the nodes that become infected in step  $\tau$ .
    - \*  $\mathcal{I}_t^\tau = \mathcal{I}_t^{\tau-1} \cup \mathcal{A}_t^\tau$ , adding the nodes that become infected in step  $\tau$ .
    - \*  $\mathcal{S}_t^\tau = \mathcal{S}_t^{\tau-1} \cup \hat{\mathcal{H}}_t^\tau \setminus \bar{\mathcal{S}}_t^\tau$ , updating the set of susceptible nodes for the next step.
    - \*  $\mathcal{H}_t^\tau = \mathcal{H}_t^{\tau-1} \setminus (\bar{\mathcal{H}}_t^\tau \cup \hat{\mathcal{H}}_t^\tau)$ , updating the set of healthy nodes for the next step.

Recall that for notational convenience, we use roman fonts to refer to sizes of sets introduced in the Edge-Revelation algorithm — for example,  $H_t^0 = |\mathcal{H}_t^0|$ ,  $B_t = |\mathcal{B}_t|$  and so on. We will refer to the natural filtration associated with the sequential procedure in the Edge-Revelation algorithm as  $\{\mathcal{F}_\tau : \tau \geq 1\}$ .

To track the evolution of the infected and susceptible vertices over the subsequent iterations of the Edge-Revelation algorithm, we make the following elementary observation. For any sequence  $a_n = o(n)$ , on the event  $\{A_t^{\tau-1} \leq a_n\}$ , we have, using Taylor expansion for the binomial probabilities:

$$\begin{aligned} \mathbb{P}[\text{Bin}(A_t^{\tau-1}, c/n) \geq 1 \mid \mathcal{F}_{\tau-1}] &= 1 - (1 - \frac{c}{n})^{A_t^{\tau-1}} = 1 - \left(1 - A_t^{\tau-1} \frac{c}{n} + O\left(\frac{(cA_t^{\tau-1})^2}{n^2}\right)\right) \\ &= (1 + o(1))A_t^{\tau-1} \frac{c}{n}. \end{aligned}$$

Similarly, on the event  $\{A_t^{\tau-1} \leq a_n\}$ ,

$$\begin{aligned}
& \mathbb{P}[\text{Bin}(A_t^{\tau-1}, c/n) \geq 2 \mid \mathcal{F}_{\tau-1}] \\
&= 1 - (1 - \frac{c}{n})^{A_t^{\tau-1}} - \frac{c}{n} A_t^{\tau-1} (1 - \frac{c}{n})^{A_t^{\tau-1}-1} \\
&= 1 - \left( 1 - A_t^{\tau-1} \frac{c}{n} + \frac{c^2}{2n^2} (A_t^{\tau-1})(A_t^{\tau-1} - 1) + o\left(\frac{(cA_t^{\tau-1})^2}{n^2}\right) \right) \\
&\quad - \frac{c}{n} A_t^{\tau-1} \left( 1 - (A_t^{\tau-1} - 1) \frac{c}{n} + O\left(\frac{(cA_t^{\tau-1})^2}{n^2}\right) \right) \\
&= (1 + o(1)) \left( \frac{(cA_t^{\tau-1})^2}{2n^2} \right).
\end{aligned}$$

The algorithm terminates at the first step  $\tau \geq 1$ , such that  $\bar{\mathcal{S}}_t^\tau \cup \bar{\mathcal{H}}_t^\tau = \emptyset$ . Upon termination at  $\tau$ , we have that  $\mathcal{I}_t^\tau = \mathcal{I}_t$ . We show that when  $t = o(n^{2/3})$ , then with high probability this algorithm terminates in  $\tau = 2$ ; moreover,  $I_t = I_t^{\tau=2} = o(n^{2/3})$  w.h.p.

We analyze the rounds of the algorithm sequentially. We start with  $\tau = 0$ , and note that  $I_t^0 = B_t = 2t = T = o(n^{2/3})$ . For  $\tau = 1$ , we get:

$$\begin{aligned}
\hat{H}_t^1 &= \text{Bin}(H_t^0, \mathbb{P}[\text{Bin}(A_t^0, c/n) = 1]), \\
\bar{H}_t^1 &= \text{Bin}(2, \mathbb{P}[\text{Bin}(A_t^0, c/n) = 1]) + \text{Bin}(H_t^0, \mathbb{P}[\text{Bin}(A_t^0, c/n) \geq 2]), \\
\bar{S}_t^1 &= \text{Bin}(S_t^0, \mathbb{P}[\text{Bin}(A_t^0, c/n) \geq 1]) = 0.
\end{aligned}$$

Direct computation yields  $\mathbb{E}[\hat{H}_t^1] = o(n^{2/3})$  and  $\mathbb{E}[\bar{H}_t^1] = o(n^{1/3})$ . Using Markov inequality, this immediately implies that  $\hat{H}_t^1 = o(n^{2/3})$  and  $\bar{H}_t^1 = o(n^{1/3})$ . This, in turn implies that

$$\begin{aligned}
S_t^1 &= S_t^0 - \bar{S}_t^1 + \hat{H}_t^1 = T = o(n^{2/3}), \quad H_t^1 = H_t^0 - \bar{H}_t^1 - \hat{H}_t^1 = \Theta(n), \\
A_t^1 &= \bar{H}_t^1 = o(n^{1/3}), \quad I_t^1 = I_t^0 + A_t^1 = o(n^{2/3}).
\end{aligned}$$

We next analyze the next round of the Edge Revelation algorithm. For  $\tau = 2$ , we have

$$\begin{aligned}
\hat{H}_t^2 &= \text{Bin}(H_t^1, \mathbb{P}[\text{Bin}(A_t^1, c/n) = 1]), \\
\bar{H}_t^2 &= \text{Bin}(H_t^1, \mathbb{P}[\text{Bin}(A_t^1, c/n) \geq 2]), \\
\bar{S}_t^2 &= \text{Bin}(S_t^1, \mathbb{P}[\text{Bin}(A_t^1, c/n) \geq 1]).
\end{aligned}$$

For any  $\varepsilon > 0$ , we have, for  $\delta_1 > 0$

$$\mathbb{P}[\hat{H}_t^2 > \varepsilon n^{1/3}] \leq \mathbb{P}[\hat{H}_t^2 > \varepsilon n^{1/3}, A_t^1 < \delta_1 n^{1/3}] + o(1) \leq \frac{\delta_1 c}{\varepsilon} + o(1),$$

where the last inequality follows using Markov inequality, conditioned on  $\mathcal{F}_1$ . We note that as  $\delta_1 > 0$  is arbitrary,  $\hat{H}_t^2 = o(n^{1/3})$ . A similar analysis reveals that  $\bar{H}_t^2 = o(1)$  and  $\bar{S}_t^2 = o(1)$ . Armed with these observations, we immediately conclude that

$$\begin{aligned}
S_t^2 &\leq 4A_t^1 + S_t^1 - \bar{S}_t^2 + \hat{H}_t^2 = o(n^{2/3}), \quad H_t^2 = H_t^1 - \bar{H}_t^1 - \hat{H}_t^1 = \Theta(n), \\
A_t^2 &= \bar{S}_t^2 + \bar{H}_t^2 = o(1), \quad I_t^2 = I_t^1 + A_t^1 = o(n^{2/3}).
\end{aligned} \tag{1}$$

The upper-bound in [1] is due to the  $4A_t^1$  term which accounts for the four neighbors of an additionally infected node (outside of  $\mathcal{B}_t$ ) on the  $\mathcal{C}_2$ . The validity of this recursion hinges crucially on the observation that with high probability, two nodes that are infected at round 2 (belonging to  $\mathcal{A}_t^2$ ) are at least distance two apart on  $\mathcal{C}_2$ . We state this assertion formally in the lemma below, and complete the proof assuming this lemma. We defer its proof to the end of the section.

**Lemma S2.2.** *With high probability as  $n \rightarrow \infty$ , no two infected vertices outside  $\mathcal{B}_t$  are neighbors on  $\mathcal{C}_2$ .*

Note that after  $\tau = 2$  steps the algorithm terminates with high probability, as there are no additional infected nodes identified. This completes the proof.  $\square$

Finally, we turn to the proof of Lemma S2.2.

*Proof of Lemma S2.2:* Note that two neighboring nodes are infected in the first two rounds of the Edge Revelation algorithm provided there exist two vertices at distance at most two on  $\mathcal{C}_2$  such that at least one is infected and the other node becomes susceptible. There are  $\Theta(n)$  such pairs, and the probability of such an event is  $\mathbb{P}(\text{Bin}(A_t^1, c/n) \geq 1)\mathbb{P}(\text{Bin}(A_t^1, c/n) \geq 2)$ . The required result follows upon computing the expected number of such neighboring pairs on  $\mathcal{C}_2$ .  $\square$

## B. Spreading time Upper-Bound for Complex Contagion.

**Theorem S2.3.** *With high probability, the entire graph will be infected in time  $n^{2/3}(\log \log n)^2(1 + o(1))$ .*

*Proof of Theorem S2.3.* We devise an algorithm to lower bound the initial growth of the set of infected nodes. Let us consider a sequence  $a_n \rightarrow \infty$  as  $n \rightarrow \infty$ , to be specified later. Next, we divide the cycle into consecutive intervals of length  $L = n^{2/3}a_n(\log \log n)^2$ . Call an interval *active* if two neighboring nodes (an adjacent pair) within that interval are infected. Initially, declare the interval containing the original seed nodes as an active interval. Starting with the initial seed nodes, after  $n^{2/3}a_n$  steps the length of the original interval grows to  $2n^{2/3}a_n$ . In general, after  $n^{2/3}a_n$  time steps the length of infected segments in each active interval will be at least  $n^{2/3}a_n$  due to the deterministic growth along the cycle. By revealing the edges of  $\mathcal{G}_{n,c/n}$  that are incident to the newly infected nodes at the end of each  $n^{2/3}a_n$  epoch, we can identify new active intervals that will, in turn, grow and activate other intervals. Formally, we consider the following algorithm to undercount the number of infected nodes. Denote by  $\mathcal{X}_\tau$  the set of active intervals after  $\tau$  epochs of length  $n^{2/3}a_n$  each, and let  $X_\tau = |\mathcal{X}_\tau|$  be the number of such intervals.

### Algorithm: Interval-Growth

- Initialize:
  - Let  $N = n/L = n^{1/3}/(a_n(\log \log n)^2)$ . Divide the cycle into  $N$  intervals of length  $L$  each, and label them by  $[N]$ ; let the initial seed nodes be contained in the interval that is labeled one:  $\mathcal{X}_0 = \{1\}$ .
- For  $\tau \geq 1$ , given  $\mathcal{X}_{\tau-1}$ :
  - Infect  $n^{2/3}a_n$  new nodes along the cycle in each of the active intervals. Add edges independently with probability  $c/n$ , connecting the newly infected nodes to the healthy nodes.
  - Update the set of active intervals by adding all intervals that have two adjacent infected nodes due to the edge exposure operation in the previous step:  $\mathcal{X}_\tau \leftarrow \mathcal{X}_{\tau-1}$ .

The following lemma derives a lower bound on the number of active intervals after  $O(\log \log n)$  steps.

**Lemma S2.4** (Initial Growth of the intervals). *For any  $C > 0$ , there exists a sequence  $t_n := t_n(C) = o(\log \log n)$  such that for*

$$\tau_n = \frac{1}{\log 3} \left( \log \log n + t_n \right),$$

*with high probability as  $n \rightarrow \infty$ ,  $X_{\tau_n} \geq Cn^{1/9}(\log n)^{1/3}$ .*

An extra  $n^{2/3}$  epoch beyond  $\tau_n$  ensures that each activated interval has at least  $n^{2/3}$  infected nodes. The next Lemma shows that this is enough to guarantee that the whole graph will be infected in  $(\tau_n a_n + 2)n^{2/3} + 2$  time.

**Lemma S2.5** (End Regime). *Let  $T_n$  be the first time that 2-complex contagion infects  $Cn^{7/9}(\log n)^{1/3}$  nodes, where  $C > 2/c$  is a universal constant. Then with high probability, all nodes are infected by time  $T_n + n^{2/3} + 2$ .*

This concludes the proof.  $\square$

It remains to prove Lemma S2.4 and Lemma S2.5. We first turn to the proof of Lemma S2.4.

*Proof of Lemma S2.4.* Let us denote the natural filtration associated with the growth process outlined in the Interval-Growth algorithm by  $\{\mathcal{F}_\tau : \tau \geq 1\}$ . Note that at the end of  $\tau - 1$  steps, we have  $X_{\tau-1}$  infected intervals, and thus  $N - X_{\tau-1}$  non-active intervals. Each non-active interval of length  $L$  has at least  $\frac{1}{2}L$  mutually disjoint adjacent pairs,

and the interval is activated if any one of these adjacent pairs is infected in the next step of the Interval-Growth algorithm introduced above. The independence of the added edges naturally implies that given  $\mathcal{F}_{\tau-1}$ , we have:

$$X_\tau = X_{\tau-1} + \text{Bin}(N - X_{\tau-1}, p_\tau),$$

where  $p_\tau$  is the conditional probability that an interval is activated by the edge exposure operation in the Interval-Growth algorithm. Given  $\mathcal{F}_{\tau-1}$  we can lower bound  $p_\tau$  as follows. Each non-active interval has at least  $\frac{1}{2}L$  disjoint adjacent pairs of neighboring nodes, and thus if the edge exposure infects a node and creates at least one infected node for its neighbor, the interval is activated due to complex contagion along the cycle. Thus we have,

$$p_\tau \geq \mathbb{P}\left[\text{Bin}\left(\frac{1}{2}L, \mathbb{P}\left[\text{Bin}\left(X_{\tau-1}n^{2/3}a_n, \frac{c}{n}\right) \geq 2\right]\mathbb{P}\left[\text{Bin}\left(X_{\tau-1}n^{2/3}a_n, \frac{c}{n}\right) \geq 1\right]\right) \geq 1\right].$$

Set  $\delta_n \rightarrow 0$  as  $n \rightarrow \infty$ . Consider a choice of  $\tau_n$  satisfying the conditions of Lemma S2.4. On the event that  $X_{\tau_n-1} > \varepsilon N$  for some  $\varepsilon > 0$ , the claim holds automatically. Thus we have, on the event  $\{X_{\tau-1} \leq N\delta_n\}$

$$\mathbb{E}[X_\tau - X_{\tau-1}] \geq \frac{1}{4}X_{\tau-1}^3(a_n c)^3.$$

Using Bernstein's inequality (lower tail bound), we have, for some universal constant  $c_0 > 0$  with probability at least  $1 - 2\exp(-c_0 a_n^3)$

$$X_\tau \geq X_{\tau-1}^3 \left(\frac{ca_n}{2}\right)^3.$$

Let us choose  $\tau_n = \frac{\log \log n + t_n}{\log 3}$  for some sequence  $t_n = t_n(C) = o(\log \log n)$ . Then using union bound, the probability that we do not have the desired growth in the number of infected intervals in at least one of the rounds may be upper bounded by  $\tau_n \exp(-c_0 a_n^3)$ . We note that if we choose  $a_n = \log \log n$ , the probability of this bad event is  $o(1)$ . Moreover, on the good event, we have,  $X_{\tau_n} \geq (\frac{ca_n}{2})^{3^{\tau_n}}$ . With  $\tau_n = (\log \log n + t_n)/\log 3$ , we can choose  $t_n$  appropriately such that  $X_{\tau_n} \geq Cn^{1/9}(\log n)^{1/3}$ . Finally, note that in  $\Theta(\log \log n)$  rounds, we grow to length  $n^{2/3}a_n \log \log n$  on the first interval, which is  $o(L)$ , thus indicating that the growth in infected vertices is sustained throughout the first  $\tau$  rounds. This establishes the desired lower bound on the number of activated intervals in the first  $\tau$  rounds.  $\square$

Finally, we prove Lemma S2.5.

*Proof of Lemma S2.5.* Fix any node  $x$  in the graph, and consider the interval  $\mathcal{L}_x$  along the  $\mathcal{C}_2$  cycle with center at  $x$  and of length  $n^{2/3}$ . We say that the interval  $\mathcal{L}_x$  contains a *susceptible pair* if it contains two neighboring vertices on  $\mathcal{C}_2$ , at least one of which is infected, and the other (possibly uninfected) has at least one additional infected neighbor. We note that if an interval contains a susceptible pair at time  $T_n$ ,  $x$  will be infected by time  $T_n + 2 + n^{2/3}$  due to complex contagion along the cycle. Thus without loss of generality, consider  $x$  such that  $\mathcal{L}_x$  does not contain a susceptible pair at time  $T_n$ . Let  $A_x$  denote the event that  $\mathcal{L}_x$  contains a susceptible pair at time  $T_n + 1$ . For any fixed  $x$ ,  $\mathcal{L}_x$  has at least  $\frac{1}{2}n^{2/3}$  disjoint pairs of adjacent vertices. Each such pair is susceptible if at least one node is infected and the other has an infected neighbor. Denoting the number of infected vertices at  $T_n$  as  $I_{T_n}$ , we observe that a fixed pair becomes susceptible by time  $T_n + 1$  with probability at least  $\mathbb{P}[\text{Bin}(I_{T_n}, \frac{c}{n}) \geq 2]\mathbb{P}[\text{Bin}(I_{T_n}, \frac{c}{n}) \geq 1]$ . The probability of the complement is thus at most  $(1 - \mathbb{P}[\text{Bin}(I_{T_n}, \frac{c}{n}) \geq 2]\mathbb{P}[\text{Bin}(I_{T_n}, \frac{c}{n}) \geq 1])$ . Using independence of the adjacent pairs in  $\mathcal{L}_x$ , we have,

$$\mathbb{P}(A_x^C) \leq \left(1 - \mathbb{P}\left[\text{Bin}\left(Cn^{7/9}(\log n)^{1/3}, \frac{c}{n}\right) \geq 2\right]\mathbb{P}\left[\text{Bin}\left(Cn^{7/9}(\log n)^{1/3}, \frac{c}{n}\right) \geq 1\right]\right)^{\frac{1}{2}n^{2/3}} = o\left(\frac{1}{n}\right),$$

for  $C > 1$  satisfying  $Cc > 2$ . Finally, a union bound over the vertices  $x$  with no adjacent infected pair in  $\mathcal{L}_x$  immediately implies that with high probability, every vertex has an infected adjacent pair within distance  $n^{2/3}$  by time  $T_n + 1$ . Thus we can guarantee that all vertices will be infected by time  $T_n + n^{2/3} + 2$ , establishing the desired result.  $\square$

### S3. Complex contagion on $\mathcal{C}_1$ union random graph with simple adoptions along $\mathcal{C}_1$ (Theorem 2)

In this section, we consider a model where in addition to complex contagion we have simple contagions along the  $\mathcal{C}_1$  edges, i.e. contagion can spread with probability  $q_n$  along  $\mathcal{C}_1$ . In this model, we compare the diffusion speed between  $\mathcal{C}_1 \cup \mathcal{G}_{n,2/n}$  and  $\mathcal{C}_2$ . We conclude that for large enough  $q_n$ , the contagion spreads faster in  $\mathcal{C}_1 \cup \mathcal{G}_{n,2/n}$ . Hence, when there is a high enough (but vanishing with increasing  $n$ ) probability of simple adoptions along the cycle-edges the rewiring of even the  $\mathcal{C}_2$  edges will speed up the spread of complex contagions.

**A. Lower-bound on the spreading time of contagion with simple adoptions.** Throughout the subsequent discussion, we denote by  $I_t$  the number of infected nodes by time  $t$ .

**Theorem S3.1** (Upper-bounding the number of infected nodes until  $t = o(\sqrt{n}/q_n)$ ). *Fix  $t = o(\sqrt{n}/q_n)$ . Then with high probability as  $n \rightarrow \infty$ ,  $I_t = o(\sqrt{n})$ .*

*Proof of Theorem S3.1.* Let  $\mathcal{B}_t$  be the largest interval on  $\mathcal{C}_1$  containing the initial seed nodes and the neighboring nodes infected by simple contagion along the cycle in time  $t$ . Denoting the size of this set by  $B_t$ , note that  $B_t$  is increasing in  $t$ ,  $B_0 = 2$  and  $B_t \rightarrow n$  with probability one as  $t \rightarrow \infty$ . To complete the proof, we will use the following lemmas.

**Lemma S3.2** (Duration of the Initial Simple Contagion Phase). *For  $tq_n = o(\sqrt{n})$ ,  $B_t = o(\sqrt{n})$ .*

**Lemma S3.3** (Initial Simple Contagion Phase). *Fix  $tq_n = o(\sqrt{n})$ . With high probability as  $n \rightarrow \infty$ , none of the nodes outside  $\mathcal{B}_t$  are infected.*

The proof of Theorem S3.1 is complete given these lemmas. We prove these assertions in the rest of this section.  $\square$

First we turn to the proof of Lemma S3.2. We will utilize the following lower tail bound on negative binomial random variables.

**Lemma S3.4** (Lower Tail Bounds for Geometric Variables). *Let  $\mathbf{g}_i, i = 1, \dots, n$  be a sequence of i.i.d. geometric variables with mean  $1/\hat{q}_n$ ,  $\hat{x} = \hat{q}_n t$  and consider  $\mathbf{G}(\hat{x}) := \sum_{i=1}^{\lfloor \hat{x} \rfloor} \mathbf{g}_i$ . If  $t\hat{q}_n \rightarrow \infty$  as  $n \rightarrow \infty$ , then  $\mathbf{G}(\hat{x}) > t/2$  with high probability.*

*Proof of Lemma S3.4.* Let  $Y_1, Y_2, \dots$  be a sequence of i.i.d. Bernoulli variables with success probability  $\hat{q}_n$ . Then  $\mathbf{G}(\hat{x})$  has the same (negative binomial) distribution as the smallest  $j$  such that exactly  $\lfloor \hat{x} \rfloor$  of  $Y_1, \dots, Y_j$  are one (see e.g. (6)). In particular,  $\mathbf{G}(\hat{x}) < t/2$  if, and only if,  $\sum_{i=1}^{\lfloor t/2 \rfloor} Y_i > \hat{x} = \hat{q}_n t$ . We can bound the probability of the latter event by a simple application of Markov inequality for the sum of i.i.d. Bernoulli variables. We have,

$$\mathbb{P} \left\{ \sum_{i=1}^{\lfloor t/2 \rfloor} Y_i > \hat{q}_n t \right\} \leq \frac{\mathbb{E} \left\{ \left( \sum_{i=1}^{\lfloor t/2 \rfloor} Y_i \right)^2 \right\}}{\hat{q}_n^2 t^2} = \frac{(t/2)\hat{q}_n}{\hat{q}_n^2 t^2} = \frac{1}{2t\hat{q}_n} = o(1).$$

Hence,  $\mathbb{P}\{\mathbf{G}(\hat{x}) \geq t/2\} \rightarrow 1$  as  $n \rightarrow \infty$ , completing the proof.  $\square$

Armed with Lemma S3.4, we can now establish Lemma S3.2.

*Proof of Lemma S3.2.* Let  $t = o(\sqrt{n}/q_n)$  and consider the spread of simple contagion along the  $\mathcal{C}_1$  edges up to time  $t$ . Starting from two adjacent seeds, the time for the simple contagion to spread to either neighboring node is a geometric random variable with success probability  $q_n$  and mean  $1/q_n$ . In particular, the time that it takes until the first of the two nodes (at either sides of the two adjacent initial seeds) gets infected is the minimum of two i.i.d. geometric mean  $1/q_n$  variables, which is another geometric variable with success probability  $\hat{q}_n = 1 - (1 - q_n)^2 = (2 + o(1))q_n$ . To upper-bound the number of simple infections up to time  $t = o(\sqrt{n}/q_n)$  we can consider a sped up infection process whereby whenever the first of the two nodes at either side of the infected interval is infected we force the second one to be infected as well. Denote the infected interval that results from this sped-up simple infection process by  $\hat{\mathcal{B}}_t$ , and set  $\hat{B}_t = |\hat{\mathcal{B}}_t|$ . First we show that  $\hat{B}_t = o(\sqrt{n})$  for  $t = o(\sqrt{n}/q_n)$ . To this end, let  $\mathbf{g}_i, i = 1, \dots, n$  be a sequence of i.i.d. geometric variables with mean  $1/\hat{q}_n$ , and  $\mathbf{x}^* := \sup\{x : \sum_{i=1}^x \mathbf{g}_i < t\}$ . The random variable  $\mathbf{x}^*$  measures the growth of  $\hat{\mathcal{B}}_t$  at both ends until time  $t$ ; hence,  $\hat{B}_t = 2 + 2\mathbf{x}^*$ . Let  $\hat{x} = 2\hat{q}_n t$  and consider  $\mathbf{G}(\hat{x}) := \sum_{i=1}^{\lfloor \hat{x} \rfloor} \mathbf{g}_i$ . Lemma S3.4 implies that  $\mathbf{G}(\hat{x}) > t$  with high probability whenever  $t\hat{q}_n \rightarrow \infty$  as  $n \rightarrow \infty$ . Thus  $\hat{B}_t = 2 + 2\mathbf{x}^* < 2 + 2\hat{x} = 2 + 4t\hat{q}_n = o(\sqrt{n})$  with high probability. Finally, we show that with high probability as  $n \rightarrow \infty$ ,  $\mathcal{B}_t \subset \hat{\mathcal{B}}_t$ . Note that  $\mathcal{B}_t \not\subset \hat{\mathcal{B}}_t$  only if

there is at least one vertex which is infected by complex contagion up to time  $t$ . We note that occurs with probability  $o(1)$  by Lemma S3.3. This establishes that  $\mathcal{B}_t \subset \hat{\mathcal{B}}_t$  with high probability. The above completes the proof for the case  $t\hat{q}_n \rightarrow \infty$ . The case  $t\hat{q}_n = O(1)$  follows from the monotonicity of  $B_t$ .  $\square$

Finally we establish Lemma S3.3.

*Proof of Lemma S3.3.* Fix  $t = o(\sqrt{n}/q_n)$  and note that Lemma S3.2 implies that there exists a sequence  $a_n = o(\sqrt{n})$  such that  $\mathbb{P}(B_t < a_n) = 1 - o(1)$ . Now, conditional on  $\{B_t < a_n\}$ , note that for contagion to spread to some node outside of  $\mathcal{B}_t$ , there has to be at least one node outside of  $\mathcal{B}_t$  that has at least two long ties to the nodes inside  $\mathcal{B}_t$ . Therefore

$$\begin{aligned} & \mathbb{P}\{\text{Some node outside } \mathcal{B}_t \text{ is infected}\} \\ & \leq \mathbb{P}\{\text{Some nodes outside } \mathcal{B}_t \text{ has two long-tie to the nodes inside } \} \\ & \leq \mathbb{P}\{\text{Bin}(n - B_t, \mathbb{P}[\text{Bin}(B_t, 2/n) \geq 2]) \geq 1\} = O\left((n - B_t) \frac{4B_t^2}{n^2}\right) = o(1). \end{aligned}$$

Hence for  $t = o(\sqrt{n}/q_n)$ , with high probability all infected nodes belong to  $\mathcal{B}_t$ , and  $\mathcal{I}_t = \mathcal{B}_t$ . This completes the proof.  $\square$

**B. Upper-bound on the spreading time of contagion with simple adoptions.** The next result derives an upper bound on the infection time of all nodes in the graph. Some aspects of the proof are similar to that of Theorem S2.3.

**Theorem S3.5.** *With high probability, the entire graph will be infected in time  $3\frac{\sqrt{n}}{q_n}(\log \log n)^2(1 + o(1))$ .*

*Proof of Theorem S3.5.* As in the proof of Theorem S2.3, we devise an algorithm to lower bound the initial growth of the set of infected nodes. Next, we divide the cycle into consecutive intervals of length  $L = \sqrt{n}(\log \log n)^3$ . Call an interval *active* if it contains an infected node. Initially, declare the interval containing the original seed nodes, an active interval. Starting with the initial seed nodes, after  $2\sqrt{n} \log \log n/q_n$  steps the length of the original interval grows to at least  $\sqrt{n} \log \log n$  with high probability. In general, with high probability as  $n \rightarrow \infty$ , over the first  $O(\log \log n)$  iterations of this algorithm, after each set of  $2\sqrt{n} \log \log n/q_n$  time steps, the length of infected segments in each active interval will grow at least  $\sqrt{n} \log \log n$  due to the simple contagion along the cycle. By revealing the edges of  $\mathcal{G}_{n,2/n}$  that are incident to the newly infected nodes at the end of each  $2\sqrt{n} \log \log n/q_n$  epoch, we can identify new active intervals that will, in turn, grow and activate other intervals. Formally, we consider the following algorithm to undercount the number of infected nodes. Denote by  $X_\tau$  the number of active intervals after  $\tau$  epochs of length  $2\sqrt{n} \log \log n/q_n$  each.

**Algorithm: Super-Exponential-Activation**

- Initialize:
  - Let  $N = \sqrt{n}/(\log \log n)^3$ . Divide the cycle into  $N$  intervals of length  $L_n = \sqrt{n}(\log \log n)^3$  each, and label them by  $[N]$ ; let the initial seed nodes be contained in the interval that is labeled one:  $\mathcal{X}_0 = \{1\}$ .
- For  $\tau \geq 1$ , given  $\mathcal{X}_{\tau-1}$ :
  - Wait for an epoch of length  $2\sqrt{n} \log \log n/q_n$  and track the growth of infected nodes along the cycle by simple contagion during this epoch.
  - Add edges independently with probability  $2/n$  connecting the new infected nodes to the healthy nodes.
- Update the set of active intervals by adding all intervals that have new infected nodes in them:  $\mathcal{X}_\tau \leftarrow \mathcal{X}_{\tau-1}$ .

The first lemma derives a lower bound on the number of active intervals after  $O(\log \log n)$  steps.

**Lemma S3.6** (Initial Growth of the intervals). *For any  $C > 0$ , there exists a sequence  $t_n := t_n(C) = o(\log \log n)$  such that for*

$$\tau_n = \frac{1}{\log 2} \left( \log \log n + t_n \right),$$

*with high probability as  $n \rightarrow \infty$ ,  $X_{\tau_n} \geq Cn^{1/4}(\log n)^{1/2}$ .*

Finally, the next result states that with high probability, the contagion process spreads to the whole graph in time  $(\tau_n)(2\sqrt{n} \log \log n / q_n) + 1 + 2\sqrt{n}/q_n$ .

**Lemma S3.7** (End Regime). *Let  $T_n$  be the first time that simple contagion infects at least  $Cn^{3/4}\sqrt{\log n}$  nodes, where  $C > 1$  is a universal constant. Then with high probability, all nodes are infected by time  $T_n + 1 + 2\sqrt{n}/q_n$ .*

The proof follows upon combining Lemma S3.6 and Lemma S3.7, and noting that  $1/\log 2 < 3/2$ .  $\square$

We turn to the proof of Lemma S3.6 and Lemma S3.7. We first establish that for the first  $O(\log \log n)$  rounds, at least  $\sqrt{n} \log \log n$  new nodes are infected over each  $2\sqrt{n} \log \log n / q_n$  epoch. To this end, we require the following lemma.

**Lemma S3.8.** *Fix  $\tau_n = \frac{1}{\log 2} \log \log n(1 + o(1))$ . With high probability as  $n \rightarrow \infty$ , every activated interval gains at least  $\sqrt{n} \log \log n$  new infected nodes over each of the first  $\tau_n$  epochs of length  $2\sqrt{n} \log \log n / q_n$ .*

*Proof of Lemma S3.8.* We begin with the observation that the waiting time for an activated interval to gain at least  $\sqrt{n} \log \log n$  new vertices via simple contagion is a sum of  $\sqrt{n} \log \log n$  i.i.d. Geometric random variables, each with mean  $1/q_n$ . Let  $\{g_1, g_2, \dots\}$  be a sequence of i.i.d. Geometric random variables with mean  $1/q_n$ . Thus during an epoch of length  $2\sqrt{n} \log \log n / q_n$ , an activated interval fails to gain at least  $\sqrt{n} \log \log n$  new infected nodes via simple contagion along the circle if  $\sum_{i=1}^{\sqrt{n} \log \log n} g_i > 2\sqrt{n} \log \log n / q_n$ . Standard upper tail bounds on sums of geometric random variables (6, Theorem 1.14) directly implies that

$$\mathbb{P}\left[\sum_{i=1}^{\sqrt{n} \log \log n} g_i > 2\frac{\sqrt{n} \log \log n}{q_n}\right] \leq \exp\left(-\frac{\sqrt{n} \log \log n}{4}\right).$$

Note that at each epoch, there are at most  $N = \sqrt{n}/(\log \log n)^3 < \sqrt{n}$  active intervals. Thus a direct union bound argument over  $O(\log \log n)$  rounds of the algorithm establishes that with high probability, each activated interval gains the desired number of infected vertices in at each epoch. It is implicit in the calculation above that the infection of new vertices is sustained as long as an active interval is not exhausted. To show this sustained growth, note that over a time epoch of length  $2\sqrt{n} \log \log n / q_n$ , the probability an active interval gains more than  $M\sqrt{n} \log \log n$  new infected vertices, for some  $M > 1$ , can be upper-bounded as follows:

$$\mathbb{P}\left[\sum_{i=1}^{M\sqrt{n} \log \log n} g_i < 2\frac{\sqrt{n} \log \log n}{q_n}\right] \leq \exp\left(-\frac{1}{2} \log M \sqrt{n} \log \log n\right),$$

where the last inequality follows using (7, Theorem 3.1). Thus for  $M > 1$  sufficiently large, by union bound over the  $N = \sqrt{n}/(\log \log n)^3$  intervals in  $\tau_n = \frac{1}{\log 2} \log \log n(1 + o(1))$  rounds, we can guarantee that at each epoch, every active interval gains at most  $M\sqrt{n} \log \log n$  many new nodes by simple infection. Hence, no active interval is exhausted in the first  $\tau_n = \frac{1}{\log 2} \log \log n(1 + o(1))$  rounds with high probability as  $n \rightarrow \infty$  (since  $L_n = \sqrt{n}(\log \log n)^3$ ). This completes the proof.  $\square$

Given Lemma S3.8, we can now prove Lemma S3.6.

*Proof of Lemma S3.6.* Let us denote the natural filtration associated with the Super-Exponential-Activation growth process as  $\{\mathcal{F}_\tau : \tau \geq 1\}$ . Note that at the end of  $\tau - 1$  steps, we have  $X_{\tau-1}$  infected intervals, and thus  $N - X_{\tau-1}$  non-active intervals. Each non-active interval is activated if at least one node has two infected neighbors in the Super-Exponential-Activation algorithm described above. The independence of the edges added naturally implies that given  $\mathcal{F}_{\tau-1}$ , we have,

$$X_\tau = X_{\tau-1} + \text{Bin}(N - X_{\tau-1}, p_\tau),$$

where  $p_\tau$  is the conditional probability that an interval is activated by the edge exposure operation in the Super-Exponential-Growth algorithm. Let  $\mathcal{E}$  denote the good event that each active interval has gained at least  $\sqrt{n} \log \log n$  new infected vertices during each epoch of length  $2\sqrt{n} \log \log n / q_n$  up to the  $\tau^{\text{th}}$  round. Observe that Lemma S3.8 implies that  $\mathbb{P}(\mathcal{E}) = 1 - o(1)$ . Now, given  $\mathcal{F}_{\tau-1}$ , we can lower bound  $p_\tau$  on the event  $\mathcal{E}$  as follows.

$$p_\tau \geq \mathbb{P}\left[\text{Bin}\left(L, \mathbb{P}\left[\text{Bin}\left(X_{\tau-1}\sqrt{n} \log \log n, \frac{2}{n}\right) \geq 2\right]\right) \geq 1\right].$$

On the event that  $X_{\tau-1} > \varepsilon N$  for some  $\varepsilon > 0$ , the claim is automatically satisfied. Thus we set  $\delta_n \rightarrow 0$  as  $n \rightarrow \infty$ , and note that on the event  $\{X_{\tau-1} \leq N\delta_n\} \cap \mathcal{E}$

$$\mathbb{E}[X_\tau - X_{\tau-1}] \geq X_{\tau-1}^2 (\log \log n)^2.$$

Using Bernstein's inequality, we have, for some universal constant  $c_0 > 0$  with probability at least  $1 - 2 \exp(-c_0 (\log \log n)^2)$

$$X_\tau \geq X_{\tau-1}^2 \left( \frac{\log \log n}{2} \right)^2.$$

Let us choose  $\tau_n = \frac{\log \log n + t_n}{\log 2}$  for some sequence  $t_n = t_n(C) = o(\log \log n)$ . Then using union bound, the probability that we do not have the desired growth in the number of infected intervals in at least one of the rounds may be upper bounded by  $\tau_n \exp(-c_0 (\log \log n)^2)$ . We note that the probability of this bad event is  $o(1)$ . Moreover, on the good event, we have,  $X_{\tau_n} \geq \left( \frac{\log \log n}{2} \right)^{2^{\tau_n}}$ . We choose  $t_n$  appropriately such that  $X_{\tau_n} \geq Cn^{1/4} \sqrt{\log n}$ . This establishes the desired lower bound on the number of infected nodes in the first  $\tau$  rounds.  $\square$

Finally we establish Lemma S3.7.

*Proof of Lemma S3.7.* For a node  $x$ , let  $\mathcal{L}_x$  denote the interval of length  $\sqrt{n}$  on the cycle centered at  $x$ . We will show that with high probability, for each  $x$ ,  $\mathcal{L}_x$  contains at least one infected node by time  $T_n + 1$ . This implies that with high probability, all vertices will be infected by time  $T_n + 1 + 2\sqrt{n}/q_n$  due to simple contagion along the cycle. This last assertion follows using upper tail concentration for a sum of geometric random variables and union bound, exactly as described in the proof of Lemma S3.8. Thus we will omit this step in the subsequent argument.

By time  $T_n$ , we have at least  $Cn^{3/4} \sqrt{\log n}$  infected nodes. If any of these infected nodes fall in  $\mathcal{L}_x$  then we are done. If not, then for any fixed  $x$ ,  $\mathcal{L}_x$  has  $\sqrt{n}$  vertices, and the probability that each such vertex has less than two infected neighbors is at most  $\mathbb{P}\left[\text{Bin}(Cn^{3/4} \sqrt{\log n}, \frac{2}{n}) < 2\right]$ . Using independence of the edges in  $\mathcal{G}_{n,2/n}$ , the probability that none of the vertices in  $\mathcal{L}_x$  is infected by time  $T_n + 1$  is at most  $\left(1 - \mathbb{P}\left[\text{Bin}(Cn^{3/4} \sqrt{\log n}, \frac{2}{n}) = 2\right]\right)^{\sqrt{n}}$ . Let  $A_x$  denote the event that none of the vertices in  $\mathcal{L}_x$  are infected by time  $T_n + 1$ . The analysis above and direct computation immediately implies

$$\mathbb{P}(A_x) \leq n^{-C}.$$

Finally, a union bound over all nodes on the cycle completes the proof, since  $C > 1$ .  $\square$

**C. Simple adoption probabilities under logit and probit Activation functions.** In Figure 4B of the main text we present the simulation results for the spreading time of complex contagion over  $\mathcal{C}_1$  union  $\mathcal{G}_{n,2/n}$  for various probabilities of simple adoptions  $q$ . Our theoretical results in Theorem 2 suggests that having  $q = \omega(1/\sqrt{n})$  is enough to ensure a faster spread in  $\mathcal{C}_1 \cup \mathcal{G}_{n,1/n}$  compared to  $\mathcal{C}_2$ . Here we derive the corresponding conditions on the parameters of the logit and probit functions to ensure that  $q = \omega(1/\sqrt{n})$  under these classes of activation functions. Consider a probit activation function such that the probability of adoptions when the number of infected neighbors is  $x$  is given by:

$$\Phi_{\theta, \sigma_n}(x) = \int_{-\infty}^{\frac{x-\theta}{\sigma_n}} \frac{1}{\sqrt{2\pi}} e^{-t^2/2} dt$$

We are interested in the asymptotic regime  $\sigma_n \rightarrow 0$  as  $n \rightarrow \infty$ . We choose  $\theta = 1.5$  to ensure a high probability of adoption with two infected neighbors and a low (but non-zero) adoption probability with only one infected neighbor. There is no adoption when there are no infections in the agent's neighborhood. The probability of adoptions below threshold is given by:

$$\hat{q}_n = \Phi_{1.5, \sigma_n}(1) = \int_{-\infty}^{-\frac{1}{2\sigma_n}} \frac{1}{\sqrt{2\pi}} e^{-t^2/2} dt = \int_{\frac{1}{2\sigma_n}}^{+\infty} \frac{1}{\sqrt{2\pi}} e^{-t^2/2} dt$$

Using the Gaussian tail bounds for  $x > 0$ ,

$$\frac{1}{\sqrt{2\pi}} \frac{x}{x^2 + 1} e^{-x^2/2} \leq \int_x^\infty \frac{1}{\sqrt{2\pi}} e^{-t^2/2} dt \leq \int_x^\infty \frac{t}{x} \frac{1}{\sqrt{2\pi}} e^{-t^2/2} dt = \frac{e^{-x^2/2}}{x\sqrt{2\pi}},$$

we get

$$\frac{e^{-1/8\sigma_n^2}}{\sqrt{2\pi}} \left( \frac{2\sigma_n}{1 + 4\sigma_n^2} \right) \leq \hat{q}_n \leq 2\sigma_n \frac{e^{-1/8\sigma_n^2}}{\sqrt{2\pi}},$$

Hence,

$$\hat{q}_n = \Theta \left( 2\sigma_n e^{-1/8\sigma_n^2} \right),$$

In particular, taking  $\sigma_n = 1/\sqrt{8 \log n^\alpha}$  yields that

$$\hat{q}_n = \Theta \left( \frac{1}{\sqrt{2 \log n^\alpha}} n^{-\alpha} \right),$$

Hence,  $\hat{q}_n = o(n^{-1/2})$  for  $\alpha \geq 1/2$  and  $\hat{q}_n = \omega(n^{-1/2})$  for  $\alpha < 1/2$ .

We can repeat the same calculations when the activation functions are specified by a logistic function:

$$\Psi_{\theta, \sigma_n}(x) = \frac{1}{1 + e^{(1/\sigma_n)(\theta - x)}}.$$

The probability of adoptions below threshold for logistic activation functions is given by:

$$\tilde{q}_n = \Psi_{1.5, \sigma_n}(1) = \frac{1}{1 + e^{(1/2\sigma_n)}} = \Theta(e^{-1/2\sigma_n}).$$

for  $\sigma_n \rightarrow 0$  as  $n \rightarrow \infty$ . Choosing  $\sigma_n = \frac{1}{2 \log(n^\alpha)}$  yields  $\tilde{q}_n = \Theta(n^\alpha)$ :  $\tilde{q}_n = o(n^{-1/2})$  for  $\alpha > 1/2$  and  $\tilde{q}_n = \omega(n^{-1/2})$  for  $\alpha < 1/2$ .

Note that  $\Phi_{\theta, \sigma}(0) > 0$  and  $\Psi_{\theta, \sigma}(0) > 0$ ; hence, the logit and probit activation functions allow for a small probability of "spontaneous" adoptions even when there are no infected neighboring nodes.

#### S4. Complex contagion over $\mathcal{C}_2^\eta$ with simple adoptions along $\mathcal{C}_1$ (Theorem 3)

Theorems S2.1 and S2.3 characterize the time needed for all nodes to be infected by 2-complex contagion on  $\mathcal{C}_2 \cup \mathcal{G}_{n, 2/n}$ . In comparison, pure complex 2-contagion on  $\mathcal{C}_4$  requires  $\Theta(n)$  time to infect all vertices, although the average degree is the same in the two cases. One could naturally envision obtaining  $\mathcal{C}_2 \cup \mathcal{G}_{n, 2/n}$  by a "re-wiring" of the edges in  $\mathcal{C}_4$ , and thus from a network intervention viewpoint, the result strongly suggests the usefulness of adding long edges to speed up the complex contagion procedure. However, any further rewiring destroys the 2-core necessary for the spread of complex contagion, and thus will actually stall the infection procedure. Theorems S3.1 and S3.5 amend this picture, and conclude that with the additional presence of a small probability of adoption below threshold, the inclusion of long edges significantly speeds up the infection procedure even by replacing the  $\mathcal{C}_2$  edges.

In this section, we adopt a more dynamical viewpoint, and interpolate between  $\mathcal{C}_2$  and  $\mathcal{C}_1 \cup \mathcal{G}_{n, 2/n}$ . To facilitate the spread of the infection process on the whole graph, we add a small probability  $q_n$  of adoption below threshold along  $\mathcal{C}_1$ . Surprisingly, our findings below indicate that initial rewiring slows down the infection process, whereas after a point, provided  $q_n$  is large enough, the infection process spreads faster compared to that of complex contagion on  $\mathcal{C}_2$ .

Formally, we consider the following interpolation model. Consider two random graph processes  $\{\mathcal{D}_\eta, \eta \geq 0\}$  and  $\{\mathcal{G}_\eta, \eta \geq 0\}$  that are coupled through the common index  $\eta \geq 0$ . For any fixed  $\eta > 0$ , the graph processes are distributed as follows.

1. Let  $\{X_{ij} : 1 \leq i < j \leq n\}$  be i.i.d. Exponential random variables with rate  $1/n^2$ . Construct  $\mathcal{G}_\eta$  with vertex set  $[n]$ , and for any  $i < j$ , we add an edge connecting the two vertices if  $\{X_{ij} < \eta\}$ . Therefore, the random graph  $\mathcal{G}_\eta$  is Erdős-Rényi with edge probability  $\mathbb{P}\{X_{ij} < \eta\} = 1 - e^{-\eta/n^2}$ .

2. Associate with every edge  $i, j$  in  $\mathcal{C}_2 \setminus \mathcal{C}_1$  an independent exponential variable  $Y_{ij}$  with mean  $2n$ . Retain edge  $i, j$  in  $\mathcal{D}_\eta \subset \mathcal{C}_2 \setminus \mathcal{C}_1$  if  $Y_{ij} > \eta$ . Thus the probability that the cycle edge  $i, j$  is removed is  $1 - e^{-\eta/2n}$ .

We will study the spread of contagion on the interpolated graph  $\mathcal{C}_2^\eta := \mathcal{C}_1 \cup \mathcal{G}_\eta \cup \mathcal{D}_\eta$  in the regime  $\eta = o(n)$ . Note that for  $\eta = o(n)$ , the expected degree of a node in  $\mathcal{C}_2^\eta$  is

$$2 + (n-3)(1 - e^{-\eta/n^2}) + 2e^{-\eta/n} = 2 + (n-3) \left( \frac{\eta}{n^2} + o\left(\frac{\eta}{n^2}\right) \right) + 2 \left( 1 - \frac{\eta}{2n} + o(\eta/n) \right) = 4 + o(\eta/n).$$

Hence, for  $\eta = o(n)$  the expected average degree in  $\mathcal{C}_2^\eta$  remain fixed and equal to four, which is the degree of nodes in  $\mathcal{C}_2$ . In this formulation,  $\eta$  is asymptotically twice the expected number of edges that are rewired to construct  $\mathcal{C}_2^\eta$  from  $\mathcal{C}_2$ .

For the subsequent analysis, we parametrize  $\eta = n^\delta$  and study the infection spread over  $\mathcal{C}_2^\eta$  in two regimes.

- (i) For  $0 < \delta < 1/2$  we show that the spread slows down with increasing  $\eta$ . In this regime, two long-ties are unlikely to land on the same node, and thus complex contagion along the long ties is blocked. On the other hand, the rewiring creates single edges along the cycle, which slows down the spread of contagion along the cycle (for a formal statement see Theorem S4.2 below).
- (ii) For  $1/2 < \delta < 1$  we show that contagion takes  $O^*(n^{3/2}/\eta + \sqrt{n}/q_n)$  time to spread. For  $\eta$  large enough,  $\sqrt{n}/q_n$  is the dominant term that fixes the spreading speed. However, for  $q_n \gg 1/\sqrt{n}$  we can specify a range of  $\eta$  for which increasing  $\eta$  increases the speed, with complex contagion spreading through the long-ties. In particular, if  $q_n = n^{-1/2+\epsilon}$ , then for  $1/2 < \delta < 1/2 + \epsilon$ , contagion spreads faster for larger values of  $\eta$  (see Theorem S4.6 below).

**A. Speed of Contagion for  $0 < \delta < 1/2$ .** We establish a lower bound on the speed of contagion for  $\delta \in (0, \frac{1}{2})$  in this section. We need the following preliminary lemmas. For any graph  $G$ , let  $\deg_{\min}(G)$  denote the minimum degree in  $G$ .

**Lemma S4.1** (Unlikely occurrence of complex contagions). *For  $\eta = o(\sqrt{n})$ ,  $\mathbb{P}(\deg_{\min}(\mathcal{G}_\eta) \geq 2) = o(1)$ .*

*Proof of Lemma S4.1.* Note that for any vertex  $i \in [n]$ , its degree in the induced subgraph is distributed as  $\text{Bin}(n, 1 - e^{-\eta/n^2})$ . Thus the probability that a fixed vertex has degree at least two is

$$\mathbb{P}(\text{Bin}(n, 1 - \exp(-\eta/n^2)) \geq 2) = O\left(\frac{\eta^2}{n^2}\right).$$

Thus the expected number of vertices with degree at least two in the subgraph induced by  $\mathcal{G}_\eta$  is  $O(\eta^2/n) = o(1)$ . This concludes the proof.  $\square$

Armed with this lemma, we can now provide a lower bound on the time to contagion in this regime.

**Theorem S4.2** (Lower-bound on the spreading time). *With high probability as  $n \rightarrow \infty$ , the total spreading time is at least  $\frac{n}{2} + \frac{\eta}{4q_n}$ .*

*Proof of Theorem S4.2.* Fix  $\delta \in (0, \frac{1}{2})$ . First, note that the number of edges deleted in  $\mathcal{C}_2 \setminus \mathcal{C}_1$  is distributed as  $\text{Bin}(n, 1 - \exp(-\frac{\eta}{2n}))$ . We denote this number as  $M_\eta$ . Next, observe that Lemma S4.1 implies that with high probability, none of the vertices may be infected by complex contagion, and the infection has to spread along the cycle. To pass each missing edge in  $\mathcal{C}_2 \setminus \mathcal{C}_1$ , one incurs an independent  $\text{Geo}(q_n)$  waiting time. Setting  $\tau$  as the time for contagion, we have,

$$\mathbb{P}\left(\tau < \frac{n}{2} + \frac{\eta}{4q_n}\right) \leq \mathbb{P}\left(\sum_{i=1}^{M_\eta} \tau_i - M_\eta < \frac{\eta}{4q_n}\right) \leq \mathbb{P}\left(\sum_{i=1}^{M_\eta} \tau_i < \frac{\eta}{4q_n}(1 + o(1))\right) + o(1),$$

where  $\{\tau_i : i \geq 1\}$  are i.i.d.  $\text{Geo}(q_n)$  random variables and the second inequality follows since  $\mathbb{E}[M_\eta] = \eta/2 = o(\eta/q_n)$ . By direct computation

$$\begin{aligned} \mathbb{E}\left[\sum_{i=1}^{M_\eta} \tau_i\right] &= \mathbb{E}[M_\eta] \mathbb{E}[\tau_i] = \frac{\eta}{2q_n}(1 + o(1)). \\ \text{Var}\left[\sum_{i=1}^{M_\eta} \tau_i\right] &= \frac{1}{q_n^2} \text{Var}(M_\eta) + \frac{1 - q_n}{q_n^2} \mathbb{E}[M_\eta] = O\left(\frac{\eta}{q_n^2}\right). \end{aligned}$$

Finally, using Chebychev's inequality, we have,

$$\mathbb{P}\left(\sum_{i=1}^{M_\eta} \tau_i < \frac{\eta}{4q_n}(1 + o(1))\right) \leq 4 \frac{\text{Var}\left[\sum_{i=1}^{M_\eta} \tau_i\right]}{\mathbb{E}^2\left[\sum_{i=1}^{M_\eta} \tau_i\right]} = O\left(\frac{1}{\eta}\right) = o(1).$$

This completes the proof.  $\square$

**B. Speed of Contagion for  $\delta \in (\frac{1}{2}, 1)$ .** Let us fix  $\delta \in (\frac{1}{2}, 1)$ . Let us first concentrate on the spread of infection along the cycle via simple or complex contagion. We initialize the process by infecting two adjacent nodes. The infection spreads via complex two contagion until an edge of  $\mathcal{C}_2$  is missing, when it pays a geometric waiting time. Thus to control how many vertices are infected over certain time periods, one needs a good control on the number of missing  $\mathcal{C}_2$  edges in any sub-interval. The following lemma provides this necessary control.

**Lemma S4.3.** *Consider an interval  $\mathcal{I}$  of length  $L$  on the cycle. Let  $\mathcal{N}(\mathcal{I})$  denote the number of missing  $\mathcal{C}_2$  edges on this segment. For  $\lambda \in (0, 1)$*

$$\mathbb{P}\left[|\mathcal{N}(\mathcal{I}) - \mathbb{E}[\mathcal{N}(\mathcal{I})]| > \lambda \mathbb{E}[\mathcal{N}(\mathcal{I})]\right] \leq 2 \exp\left(-\frac{\lambda^2}{3} \mathbb{E}[\mathcal{N}(\mathcal{I})]\right).$$

*Proof of Lemma S4.3.* We observe that for any fixed interval  $\mathcal{I}$  of length  $L$ , the number of missing cycle edges  $\mathcal{N}(\mathcal{I}) \sim \text{Bin}(L, 1 - \exp(-\eta/2n))$ . The thesis follows by a direct application of Chernoff inequality for Binomial random variable.  $\square$

Given Lemma S4.3, we can turn to deriving a lower bound on the spreading time for the infection on the cycle.

**Theorem S4.4** (High probability lower-bound on the spreading time). *Fix  $t = o(\sqrt{n}/q_n + n^{3/2-\delta})$ . With high probability as  $n \rightarrow \infty$ , the number of infected vertices is  $o(n^{3/2-\delta})$ .*

*Proof of Theorem S4.4.* Fix  $t = o(\sqrt{n}/q_n + n^{3/2-\delta})$ . For any  $\varepsilon > 0$ , consider an interval of length  $L = \varepsilon n^{3/2-\delta}$  centered at the seed nodes. Denote this interval as  $\mathcal{I}$  and let  $\mathcal{N}(\mathcal{I})$  denote the number of missing cycle edges in this interval. Recalling  $\eta = n^\delta$ , we observe that  $\mathcal{N}(\mathcal{I}) \sim \text{Bin}(L, 1 - \exp(-\eta/2n))$  and thus  $\mathbb{E}[\mathcal{N}(\mathcal{I})] = L \frac{\eta}{2n} (1 + o(1)) = \varepsilon \sqrt{n}/2 (1 + o(1))$ . Thus we have, by Lemma S4.3

$$\mathbb{P}\left[\mathcal{N}(\mathcal{I}) > \frac{1}{2} \mathbb{E}[\mathcal{N}(\mathcal{I})]\right] \geq 1 - 2 \exp\left(-\frac{\varepsilon}{24} \sqrt{n}\right).$$

Note that the waiting time for the simple contagion along the cycle edges to cover the interval  $\mathcal{I}$  is distributed as  $\sum_{i=1}^{\mathcal{N}(\mathcal{I})} g_i$ , where  $\{g_i : i \geq 1\}$  are iid geometric random variables with mean  $1/q_n$ . For  $\delta > 0$  small enough, using (7, Theorem 3.1), we have,

$$\mathbb{P}\left[\sum_{i=1}^{\mathcal{N}(\mathcal{I})} g_i < \delta \frac{\mathcal{N}(\mathcal{I})}{q_n} \mid \mathcal{N}(\mathcal{I})\right] \leq \exp\left(-\frac{\delta}{2} \mathcal{N}(\mathcal{I})\right).$$

Thus with high probability as  $n \rightarrow \infty$ , for simple contagion along the cycle to cover  $\mathcal{I}$ , the waiting time to cross the single edges is at least  $\varepsilon \delta \sqrt{n}/4q_n$ . Further, Lemma S4.3 implies that the number of missing  $\mathcal{C}_2$  edges is  $O(\sqrt{n} \log n)$  with high probability. As a consequence, for  $\delta < 1$ ,  $n^{3/2-\delta} - \mathcal{N}(\mathcal{I}) = n^{3/2-\delta}(1 - o(1))$  with high probability. For complex contagion to spread along the cycle, the spreading time required is  $\Theta(n^{3/2-\delta})$  with high probability. Thus in time  $t = o(\sqrt{n}/q_n + n^{3/2-\delta})$ , with high probability as  $n \rightarrow \infty$ , contagion along the cycle covers only a subset of the vertices in  $\mathcal{I}$ .

Finally, we will prove that with high probability as  $n \rightarrow \infty$ , no vertex outside  $\mathcal{I}$  is infected by complex contagion along the long ties. To this end, note that a vertex is infected if it has at least two edges to the infected nodes. The probability of infection of each node is upper bounded by  $\mathbb{P}[\text{Bin}(L, 1 - \exp(-\eta/n^2)) \geq 2]$ . Thus the expected number of infected vertices is at most  $n \mathbb{P}[\text{Bin}(L, 1 - \exp(-\eta/n^2)) \geq 2] = O(\varepsilon^2)$ . The required claim follows using Markov inequality, once we note that  $\varepsilon > 0$  is arbitrary. This completes the proof.  $\square$

The following is an immediate consequence of Theorem S4.4 to lower-bound the spreading time for all values of  $1/2 < \delta < 1$ .

**Corollary S4.5** (Lower-bounding the spreading time). *For any  $\varepsilon > 0$  and  $1/2 < \delta < 1$  with high probability as  $n \rightarrow \infty$ , up to time  $n^{1/2-\varepsilon}/q_n$ , the number of infected nodes is at most  $\sqrt{n}$ .*

The next theorem derives an upper bound to the spreading time for the infection in the regime  $\frac{1}{2} < \delta < 1$ .

**Theorem S4.6** (High probability upper-bound on the spreading time). *Fix  $\delta \in (\frac{1}{2}, 1)$ . Then with high probability as  $n \rightarrow \infty$ , all nodes are infected by time  $3(\sqrt{n}/q_n + n^{3/2-\delta})(\log \log n)^2(1 + o(1))$ .*

*Proof of Theorem S4.6.* The proof is similar to that of Theorem S3.5 and thus we only sketch the proof, focusing on the differences. The proof again proceeds in two stages— in the first stage, we lower bound the growth of infected nodes in the original process and establish that  $\Theta(n^{5/4-\delta/2}\sqrt{\log n})$  vertices are infected in about  $O((n^{3/2-\delta} + \sqrt{n}/q_n) \log \log n)$  steps. An independent argument establishes that all vertices are infected in  $O(n^{3/2-\delta} + \sqrt{n}/q_n)$  additional time. Formally, we establish the following results.

**Lemma S4.7.** *For any fixed  $\delta \in (\frac{1}{2}, 1)$  and  $C > 1$ , there exists a sequence  $t_n := t_n(C, \delta) = o(\log \log n)$  such that with high probability as  $n \rightarrow \infty$ , the infection spreads to  $Cn^{5/4-\delta/2}\sqrt{\log n}$  nodes in at most  $3(n^{3/2-\delta} + \sqrt{n}/q_n) \log \log n(\log \log n + t_n)$  steps.*

**Lemma S4.8.** *Let  $T_n$  be the first time when the contagion infects  $Cn^{5/4-\delta/2}\sqrt{\log n}$  nodes, where  $C > 1$  is a universal constant. Then with high probability, all nodes are infected by time  $T_n + 2(\frac{\sqrt{n}}{q_n} + n^{3/2-\delta})$ .*

The proof follows.  $\square$

*Proof of Lemma S4.7.* As before, we divide the  $[n]$  nodes into  $N$  equal intervals of length  $L = n^{3/2-\delta}(\log \log n)^3$  each. We call an interval *active* if it contains at least one infected node. At time zero, we call the interval containing the original infected nodes active. We will undercount the original growth of infected vertices by a more tractable growth process. To this end, we look at the infection process at epochs of size  $(n^{3/2-\delta} + \sqrt{n}/q_n) \log \log n$ , and index the epochs by  $\tau \geq 1$ . During each epoch, the active intervals gain new infected nodes due to infections (simple and complex contagions) along the cycle edges. At the end of an epoch, we expose the long range random edges. This in turn, leads to new active intervals, and provides a lower bound on the growth of infected nodes in the original process. We denote the natural filtration associated with the undercounting process as  $\mathcal{F}_\tau$ , and let  $X_\tau$  denote the number of active intervals after  $\tau$  epochs. In each epoch, with high probability, an infected node further infects its neighbor within  $2 \log n/q_n$  time. Once we have two neighboring infected vertices, infection spreads along the cycle via simple and complex contagion. Consider the one-sided interval of length  $\frac{1}{2}n^{3/2-\delta} \log \log n$  on any active interval (to one side if the infected segment on the active interval). Lemma S4.3 implies that with (exponentially) high probability, the maximum number of missing cycle edges is  $\frac{1}{2}\sqrt{n} \log \log n$ . The total weight time to cross these missing edges is  $\sqrt{n} \log \log n/q_n$ , with (exponentially) high probability. Union bound provides that, with high probability, the contagion process along the cycle infects at least  $\frac{1}{2}n^{3/2-\delta} \log \log n$  new nodes in each active interval in each epoch of size  $(n^{3/2-\delta} + \sqrt{n}/q_n) \log \log n$ . Note that given  $\mathcal{F}_{\tau-1}$ ,

$$X_\tau - X_{\tau-1} = \text{Bin}(N - X_{\tau-1}, p_\tau).$$

where  $p_\tau$  is the conditional probability of activation of an inactive interval due to the edge-exposure step at this round. We can lower bound this probability as

$$p_\tau \geq \mathbb{P}\left[\text{Bin}\left(L, \mathbb{P}\left[\text{Bin}\left(\frac{X_{\tau-1}}{2}n^{3/2-\delta} \log \log n, 1 - \exp(-\eta/n^2)\right) \geq 2\right]\right) \geq 1\right].$$

Thus conditional on  $\mathcal{F}_{\tau-1}$ , we have the lower bound

$$\mathbb{E}[X_\tau - X_{\tau-1}] \geq (N - X_{\tau-1})L\left(\frac{X_{\tau-1}}{2}n^{3/2-\delta} \log \log n\left(\frac{\eta}{n^2}\right)\right)^2 \geq \frac{1}{8}X_{\tau-1}^2(\log \log n)^2$$

Using Bernstein inequality, we can guarantee that this growth is sustained over the first  $O(\log \log n)$  epochs leading to  $X_{\tau_n} > Cn^{\delta/2-1/4}\sqrt{\log n}$ , for  $\tau_n = (\log \log n + t_n)/\log 2$  and appropriate choice of  $t_n = t_n(C, \delta) = o(\log \log n)$ , exactly as outlined in the proof of Lemma S3.6. The proof now follows using the same arguments as outlined in the proof of Lemma S3.6.  $\square$

*Proof of Lemma S4.8.* Fix a node  $x$  and let  $\mathcal{L}_x$  be the interval of length  $L = n^{3/2-\delta}$  centered at  $x$ . The probability that any fixed vertex in this interval has at least two infected neighbors is at least  $\mathbb{P}[\text{Bin}(Cn^{5/4-\delta/2}\sqrt{\log n}, 1 - \exp(-\eta/n^2)) \geq 2]$ . Using independence of the edges, the probability that no vertex in the interval has at least two infected neighbors

is at most  $(1 - \mathbb{P}[\text{Bin}(Cn^{5/4-\delta/2}\sqrt{\log n}, 1 - \exp(-\eta/n^2)) = 2])^{n^{3/2-\delta}}$ . Denoting this event as  $A_x$ , simple computations implies that,

$$\mathbb{P}(A_x) \leq n^{-C}$$

for  $C > 1$ . By a union bound, with high probability, each node has at least one infected node in the interval of length  $L$  surrounding it. With exponentially high probability, an infected node further infects its neighbor within  $2 \log n/q_n$  time. Using union bound (over  $n$  choices of  $x$ ), in  $2(\log n)/q_n$  additional time, every interval  $\mathcal{L}_x$  will have two neighboring infected vertices and infection spreads throughout the  $\mathcal{L}_x$  intervals via simple and complex contagion. Next note that using Lemma S4.3 and a union bound over  $x$ , the maximum number of missing  $\mathcal{C}_2 \setminus \mathcal{C}_1$  edges in any interval  $\mathcal{L}_x$  is at most  $\sqrt{n}$ . Further, an application of (6, Theorem 1.14) and union bound (over  $x$ ) implies that the total passage time across the missing edges in any interval  $\mathcal{L}_x$  is at most  $2\sqrt{n}/q_n$ . Finally, complex contagion covers the remaining part of each interval in less than  $n^{3/2-\delta}$  steps. Thus with high probability, the entire graph is infected by time  $T_n + 2(\sqrt{n}/q_n + n^{3/2-\delta})$ .  $\square$

**C. Simulation results allowing for simple adoptions along all edges.** Figure S2 is a redone of the simulation results presented in Figure 4C of the main text, allowing for simple contagion probability  $q$  along all edges in the network. Both figures reveal the same kind of qualitative behavior in that, rewiring accelerates the spread for large enough values of  $q$ . Moreover, comparisons of the two figures reveal interesting consequences of the handicap assumption that we impose on the model in Figure 4C, by allowing simple contagions only along the  $C_1$  edges.

Not only the spread is accelerated for much smaller values of simple adoption probability ( $q \geq 0.0129$ ) in Figure S2 compared to Figure 4C, but also the initial slow down phase is no longer present in Figure S2. To the contrary, the first few rewired edges are the most effective in accelerating the spread: we observe diminishing returns in the acceleration (or deceleration) of contagion with the number of rewired edges in Figure S2.

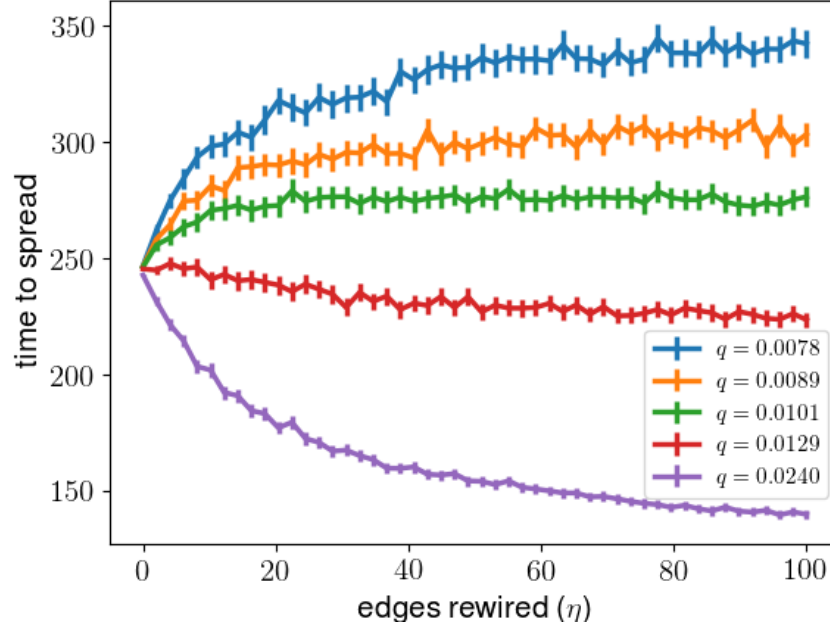

**Fig. S2.** Spreading time of complex contagion over  $C_2^\eta$  random graphs with  $n = 500$ , allowing for simple contagion with probability  $q$  along all edges (not just  $C_1$ ). Each point is the average of 1000 random draws and the error bars show the 95% normal confidence intervals around the means.

## S5. Simulations with empirical networks data

We expand on the results of simulations that we present in the main text (Figure 6) by providing additional statistics and measurements over these networks. Moreover, we provide simulations with variations of the original model to verify the robustness of our claims to changes in the model. We use four datasets that contain empirical social networks for (i) 175 rural Chinese farm villages being encouraged to sign up for insurance (8), (ii) the union of the friendship and the health advice networks collected from 17 rural villages in Uganda (9), (iii) 77 village social networks collected in the study of participation in a microfinance program in South India (10), and (iv) the Facebook friendship social networks in U.S. universities and colleges (11), from which we choose the 40 smallest networks. Table S1 summarizes the network size statistics in all these datasets. For each social network in these datasets we are interested in how interventions that modify the network structure would affect the spread of contagion. We consider three intervention strategies: (i) random rewiring, (ii) adding new edges uniformly at random, (iii) adding new edges at random with probability proportional to the number of open triads that each new edge would close. Following the same conventions as in Figure 6 of the main text, we use black, orange, blue, and red colors to plot the values corresponding to the original network, as well as the modified networks under rewiring, triad-closing and random edge additions. The plots in Figure S3 are produced in the same way as Figure 6B of the main text. The latter is simulated over the 175 social networks in the Cai et al. (8) dataset, whereas in Figure S3 we use the other three datasets with fewer social networks — Chami et al. (9), Banerjee et al. (10), and Traud et al. (11).

**Table S1. Size statistics for the empirical networks data**

| dataset              | number of networks | min size | max size | median size | mean size |
|----------------------|--------------------|----------|----------|-------------|-----------|
| Cai et al. (8)       | 175                | 13       | 117      | 51.5        | 54.03     |
| Chami et al. (9)     | 17                 | 65       | 372      | 184         | 202.12    |
| Banerjee et al. (10) | 77                 | 75       | 341      | 189         | 192.63    |
| Traud et al.(11)     | 40                 | 762      | 7677     | 3745        | 4153.82   |

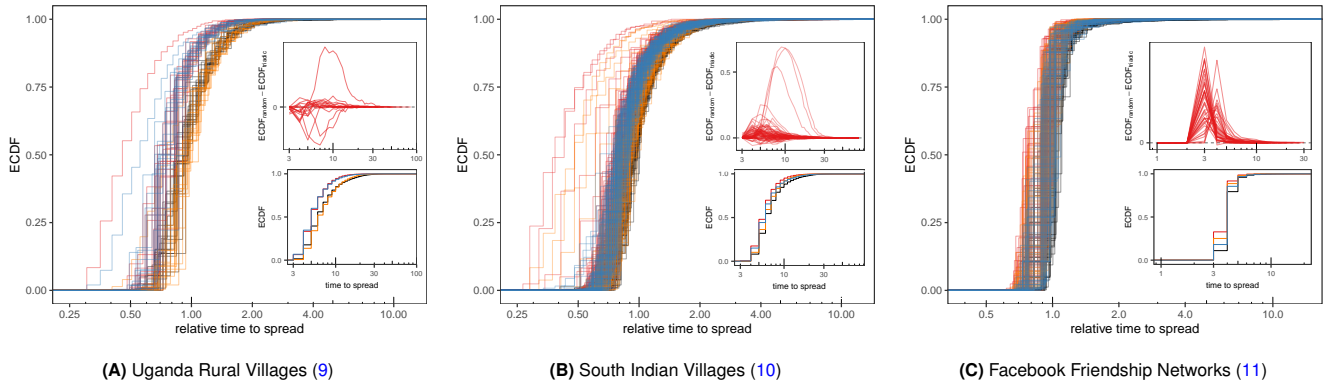

**Fig. S3.** We replicate the plots in Figure 6B of the main text (that was simulated on social network data from Chinese farm villages (8)) for three other datasets.

In any given network, starting from two randomly chosen seeds (initially infected nodes) we measure the time until 90% of the nodes are infected. Under each intervention and model of contagion that we are considering, we draw 500 random spreading time samples over the original or modified networks and compare the spreading times in terms of their empirical cumulative distribution functions (ECDFs). On a few occasions we combine these samples for all the villages over the entire dataset and compare the overall ECDFs under each intervention: Figures S5, S6, as well as the bottom left insets in Figure S3, and the second and forth rows in Figure S7 are generated this way. The intervention sizes are measured in terms of the percent of edges in the original networks, and unless otherwise specified, the intervention size is fixed at 10%: Figure 6 in the main text, as well as Figures S5 and S8, here, follow this convention. When varying the intervention size, we group the samples by their intervention size. The intervention size in each group is fixed at 5, 10, 15, 20 or 25%: Figures S6 and S7 are generated in this manner. In the first and third rows of Figure S7 we have overlaid the ECDFs of spreading times for each social network in the respective datasets (77 villages from the south Indian dataset (10) in the first row, and 17 villages from the Ugandan dataset (9) in the third row). In these two cases (the first and third rows of Figure S7) since different village sizes affect the time

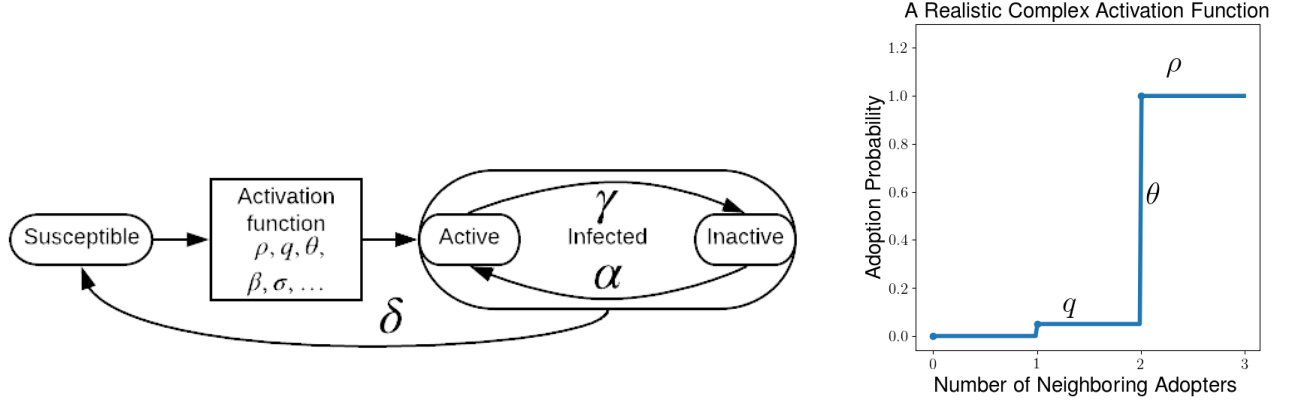

Fig. S4. The model

to 90% spread, we normalize the spreading times relative to the mean spread time in the original village (with no interventions); moreover, we put the x-axis in logarithmic scale to symmetrize the ratios below and above one.

Figure S4 shows the block diagram of the model that we have implemented for each agent in our simulations. The active and inactive infected states describe a situation where adopter agents may transition into a state where they are not effective in turning their neighboring non-adopters into adopters. We refer to this state as an inactive infected state and allow infected agents to transition back and forth between active and inactive states with probabilities  $\alpha$  and  $\gamma$  as depicted in Figure S4. In the basic model that we study in the main text all infected agents are regarded as active; hence,  $\alpha = 1$  and  $\gamma = 0$ . In general, we also allow a probability  $\delta$  for infected agents to transition back into the susceptible state; however, in our studies we set  $\delta = 0$ , as motivated by applications where infection connotes product purchase.

The activation function block determines the type of contagion (simple or complex). Different models of contagion are characterized by different parameters. For example, the simple contagion activation functions shown in Figure 1 of the main text are parametrized by the independent transmission probabilities ( $\beta$ ) along each edge. The probability of infection with  $x$  infected neighbors under this simple contagion activation function is given by  $1 - (1 - \beta)^x$ . On the other hand, the complex contagion activation function shown in Figure S4, on the right, is parametrized by a threshold value  $\theta$ , adoption probability above threshold  $\rho$ , and adoption probability below threshold  $q$ . Similarly, logit and probit activation functions studied in Section S3C are characterized by a threshold  $\theta$  and noise (or “rationality”) level  $\sigma$ . Unless otherwise specified, we compute the spreading time samples under the (0.05, 1) model from Figure S5A ( $\rho = 1$ ,  $q = 0.05$ ,  $\alpha = 1$ ,  $\gamma = 0$ ,  $\theta = 2$ ): the spreading time samples in Figures S7 and S8, here, as well as Figure 6 of the main text are all generated under the (0.05, 1) model.

In special cases (Figure S5D, here, and Figure 4C in the main text) we make a distinction between what edges pass simple contagion adoptions (probability  $q$ ) and what edges do not. Such models are not fully specified by the choice of activation functions and transition probabilities  $\alpha$ ,  $\gamma$ , and  $\delta$ , since we need to take into account the type of network edges along which transitions occur. In Figure S5D, we allow the simple contagion probability  $q$  only if the edge connecting the adopter and non-adopter agent is existent in the original network. Spreading time samples for this model are collected only under the edge addition interventions (random versus triad-closing). In Figure 4C of the main text we consider the spreading time over  $\mathcal{C}_2^n$  random graphs and allow for simple contagion probability  $q$  only along the  $\mathcal{C}_1$  cycle edges.

Figure S5 shows the overall ECDFs (combining all samples across all villages with 500 random samples per village) of the spreading times over the Chinese farm villages dataset (8). We present the results for six different models and activation function settings with 10% sized interventions. A more fine-grained version of this data where intervention sizes are varied between 5, 10, 15, 20, and 25% is presented in Figure S6. The two models labeled by (0.05, 1(0.05, 0.5)) and (0.001, 1) in Figures S5C and S5F (see the Figure captions for the corresponding model parameters) are significantly slower. In their ECDFs, we can identify a fast and a slow regime which we attribute to complex and simple contagions, respectively. If the 90% spread is reliant on complex contagion, then the spreading time samples are visibly discrete and the total spread is achieved fast. If, on the other hand, a significant number of nodes are infected through simple contagion (coin flips with probability  $q$ ), then contagion is slow and spreading time samples cover a wide range, resulting in a smooth section in the ECDF curve.

In contrast, the fractional threshold model that is labeled by REL(0.05, 1) in Figure S5E is significantly faster; its

ECDF is visibly discrete and does not contain a smooth, slow section. Under this fractional model a node is infected with high probability ( $\rho = 1$ ) if the majority of its neighbors are adopters ( $\theta^* = 0.5$ ); in particular, a leaf node with only one neighbor becomes an adopter as soon as its neighbor adopts. This is in contrast to the absolute threshold model  $\theta = 2$  where a leaf node can only be infected through the slow simple contagion (coin flips) with probability  $q$ .

In Figure S7 we present the ECDFs of the spreading times over the south Indian (10) and Ugandan (9) villages for different intervention sizes (the intervention size in Figure S3 was fixed at 10%). To further demonstrate the stochastic dominance relation between the spreading times (as random variables) under various interventions, in Figure S8 we present the difference between the ECDFs with 10% interventions for all the social networks in our four datasets. The spreading samples in both Figures S7 and S8 are generated under the  $(0.05, 1)$  model from Figure S5A ( $\rho = 1$ ,  $q = 0.05$ ,  $\alpha = 1$ ,  $\gamma = 0$ ,  $\theta = 2$ ). If the positive difference persists throughout the entire support of two ECDFs, then we conclude the stochastic dominance relation between their respective random variables.

In Figure S9 we plot the mean time to spread versus the intervention size for random and triadic edge additions. We can thus answer how much larger does the intervention size for triadic addition have to be before it is faster than random addition in each set of empirical networks. For example, Figure S9A indicates that in the Cai et al. dataset even with 25% additional triad-closing ties the mean spread time is still slower than in the networks with 10% additional random ties.

In all these measurements, we observe the same direction (sign) for the effect of interventions on the spreading time: (i) rewiring speeds up the spread of contagion compared to the original networks, (ii) contagion spreads faster in the networks with added edges compared to the original networks, (iii) contagion spreads faster in the network with added random edges compared to the network with added triad-closing edges. The magnitude of differences are larger for larger interventions.

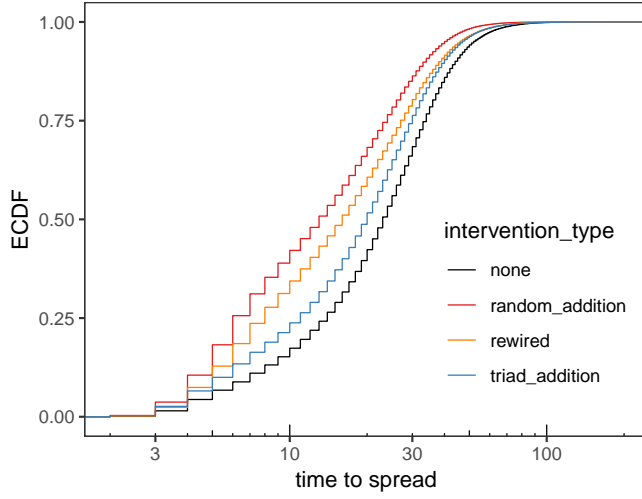

(A)  $(0.05, 1) : \rho = 1, q = 0.05, \alpha = 1, \gamma = 0, \theta = 2$

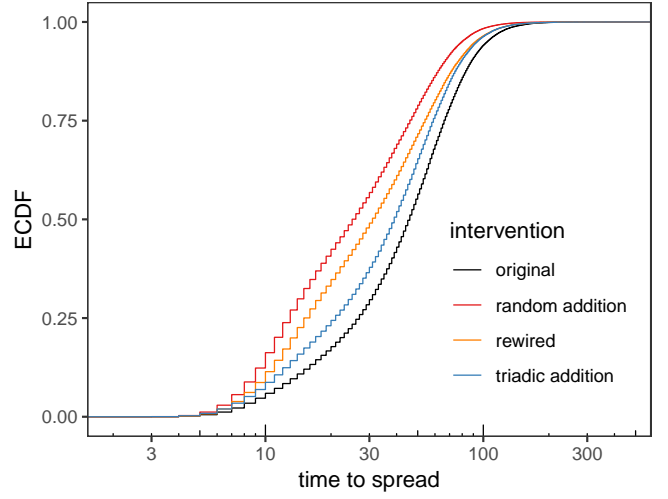

(B)  $(0.025, 0.5) : \rho = 0.5, q = 0.025, \alpha = 1, \gamma = 0, \theta = 2$

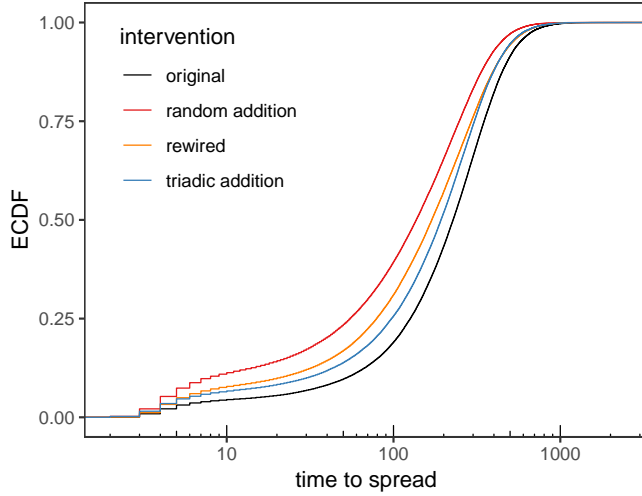

(C)  $(0.05, 1(0.05, 0.5)) : \rho = 1, q = 0.05, \alpha = 0.05, \gamma = 0.5, \theta = 2$

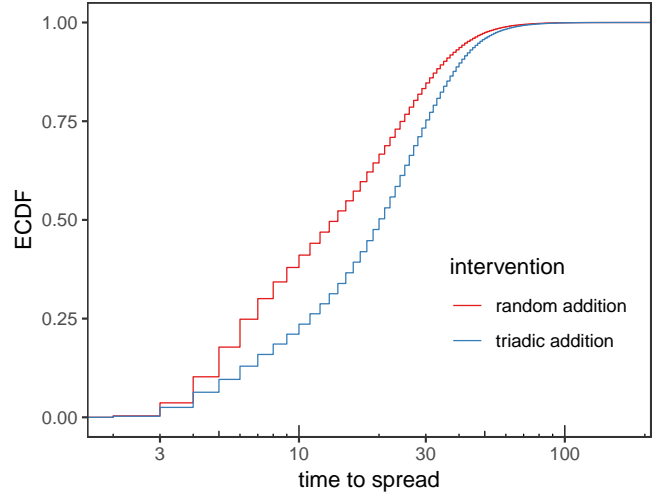

(D)  $(ORG-0.05, 1) : \rho = 1, q = 0.05, \alpha = 1, \gamma = 0, \theta = 2$ , simple adoptions happen only along the original edges and spreading time samples are collected only under edge addition interventions (triadic vs random)

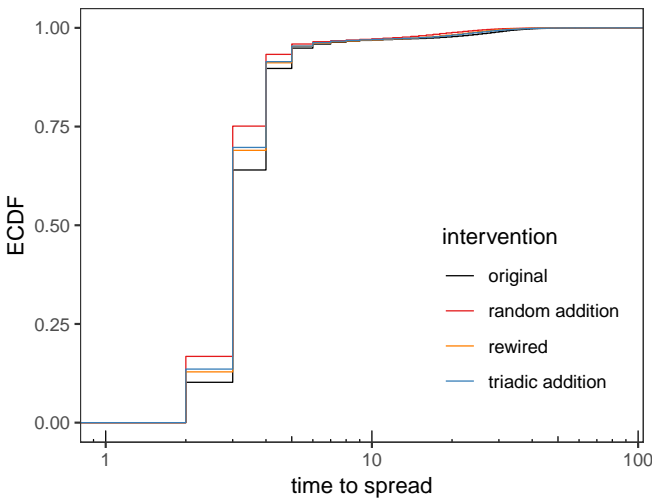

(E)  $REL(0.05, 1) : \rho = 1, q = 0.05, \alpha = 1, \gamma = 0, \theta^* = 0.5$ , complex contagion with fixed common fractional threshold ( $\theta^*$ )

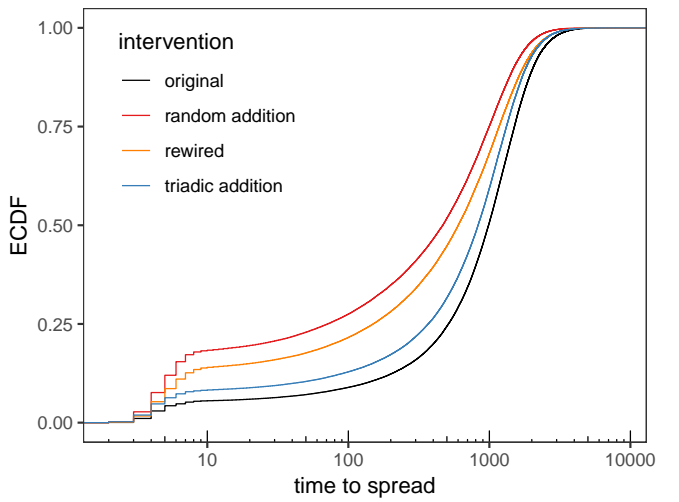

(F)  $(0.001, 1) : \rho = 1, q = 0.001, \alpha = 1, \gamma = 0, \theta = 2$

Fig. S5. The overall ECDF for the spreading times over Chinese farm villages (8) under different contagion models and interventions with fixed size (10%)

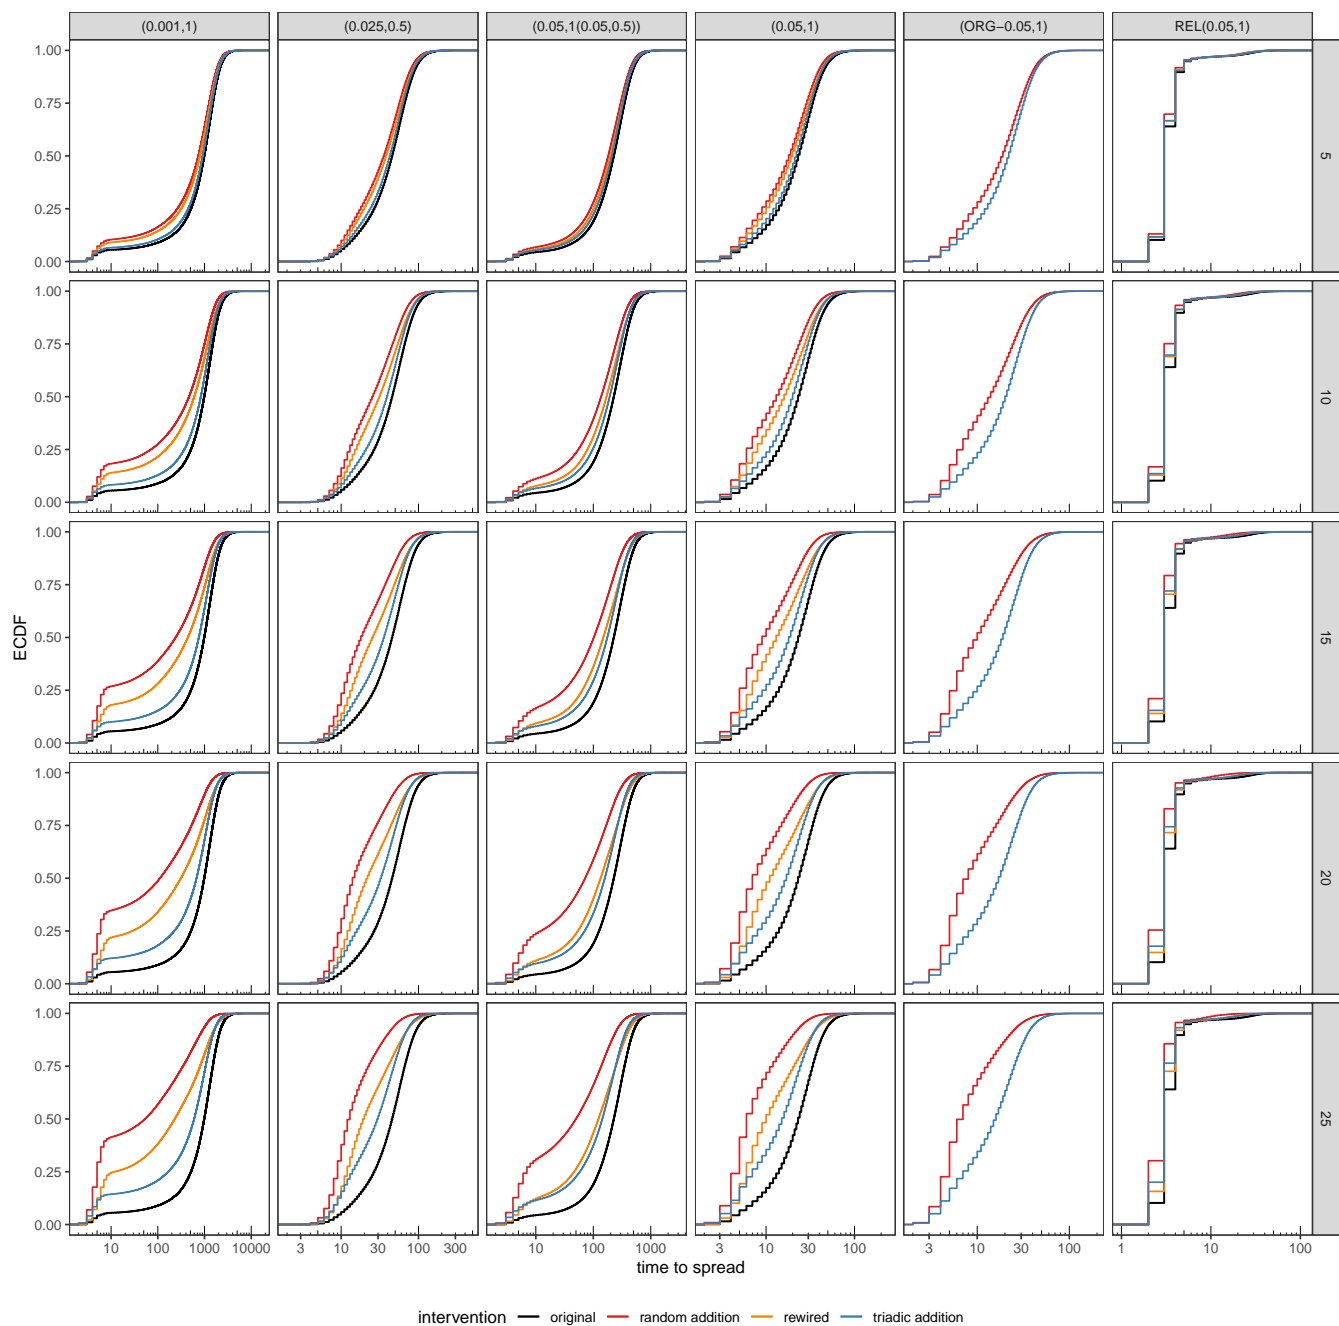

**Fig. S6.** Overall ECDFs under various interventions grouped by the intervention sizes and contagion models for the Chinese farming villages (8). The model labels at the top are as introduced in the captions of Fig. S5. The intervention sizes are shown on right side.

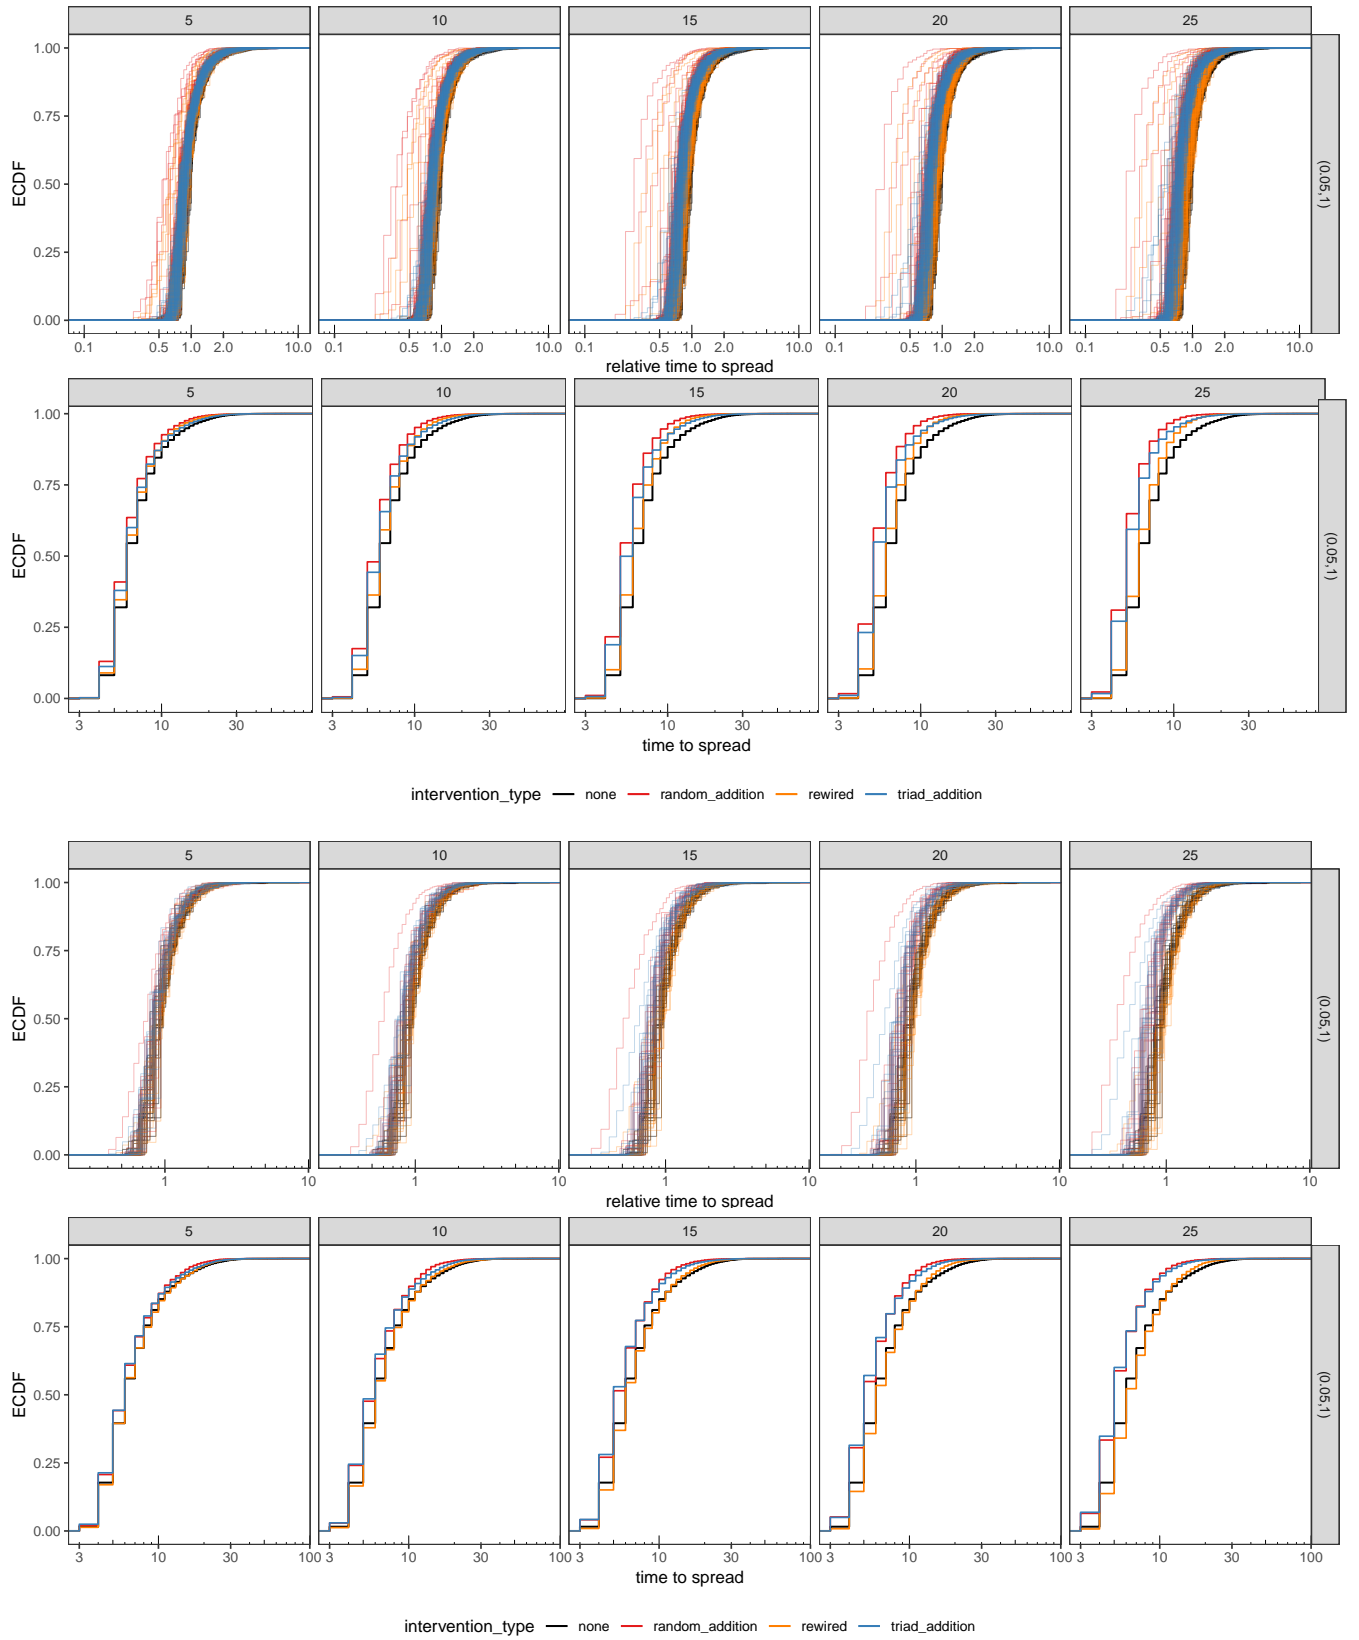

**Fig. S7.** ECDFs under various interventions grouped by the intervention size for the South Indian (10, top two) and Ugandan (9, bottom two) villages. For each dataset, the top figures show the ECDFs for the individual villages (overlaid) and the bottom figures combine the random samples (spreading times) over the entire dataset. These figures follow the same conventions as Figure 6 of the main text.

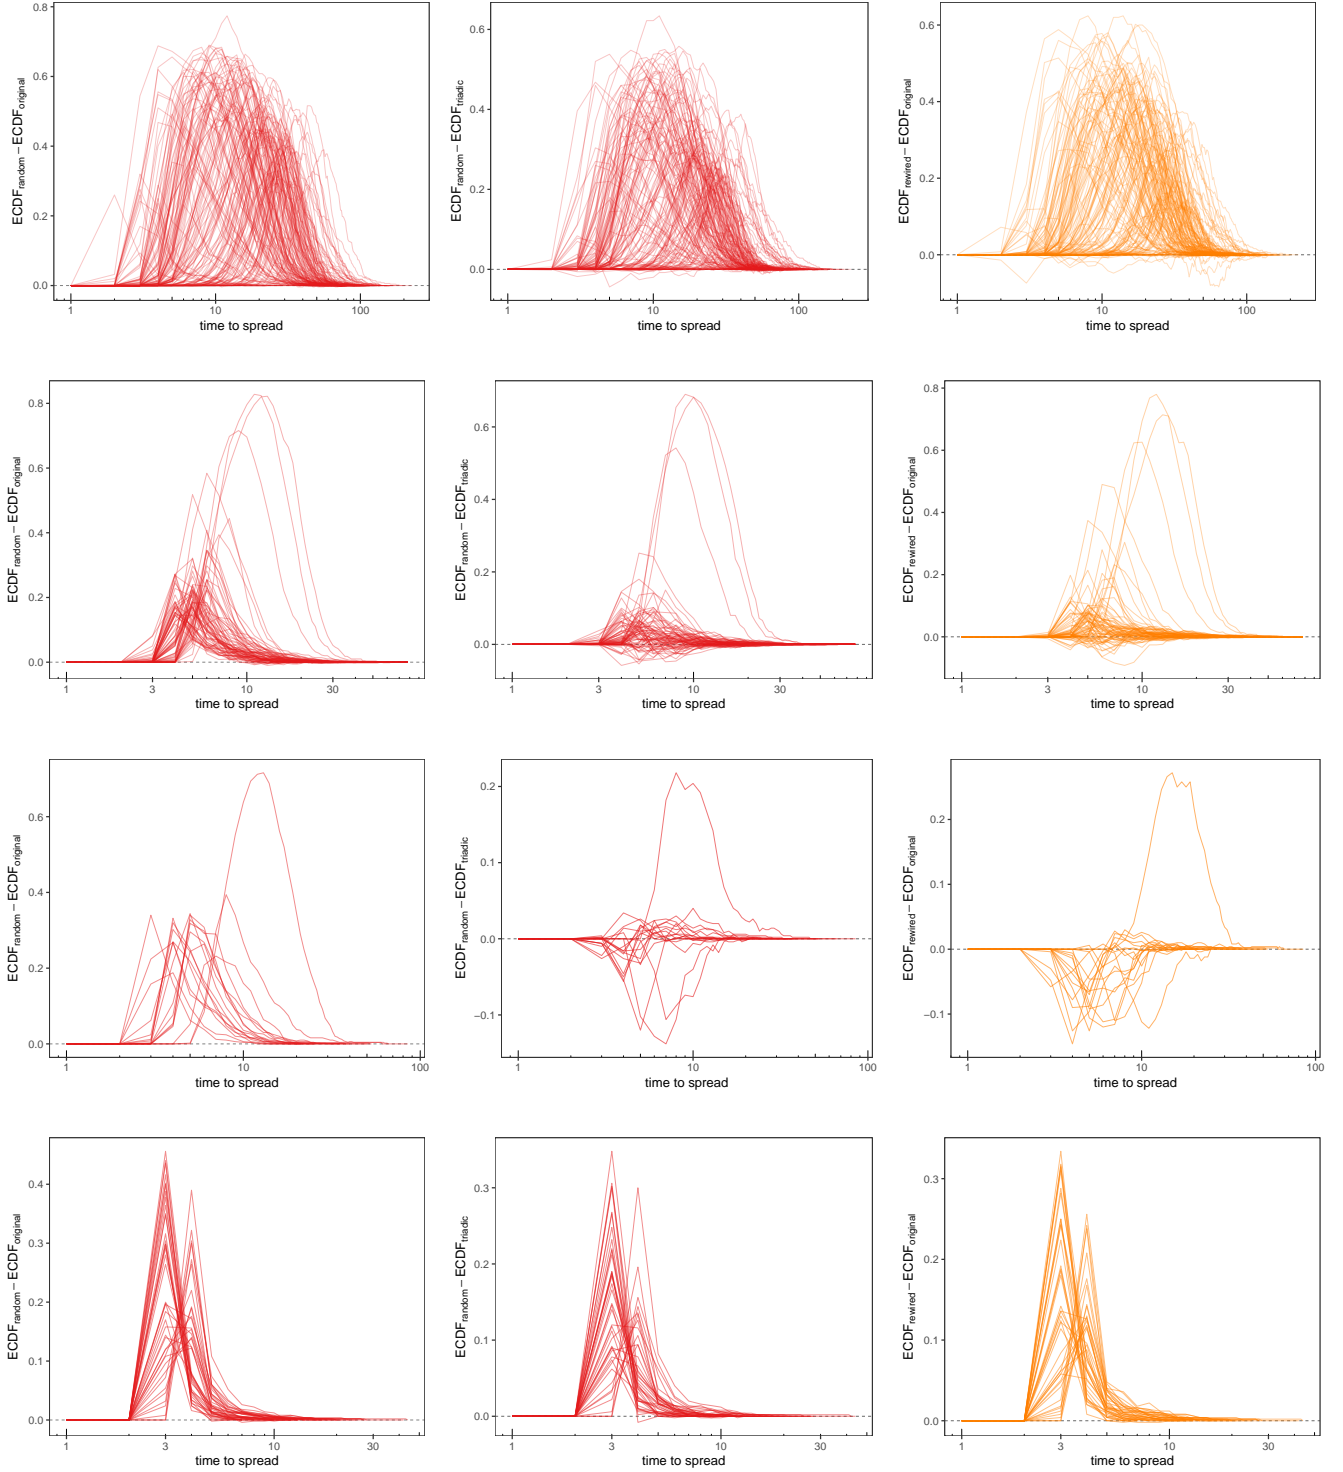

**Fig. S8.** Difference between spreading time ECDFs in networks with 10% additional random edges and the original ones (leftmost), between the networks with 10% additional random and triad closing edges (middle), and between the 10% rewired and the original networks (rightmost), for rural villages in China (8) — first row, South Indian (10) — second row, and Uganda (9) — third row, as well as the Facebook social networks (11) — fourth row. The positive differences indicate the stochastic dominance relation between the spread times (as random variables) under one intervention over another. The spreading time samples are computed under the  $(0.05, 1)$  model from Figure S5A with  $q = 0.05$ ,  $\alpha = 1$ ,  $\gamma = 0$ , and  $\theta = 2$ .

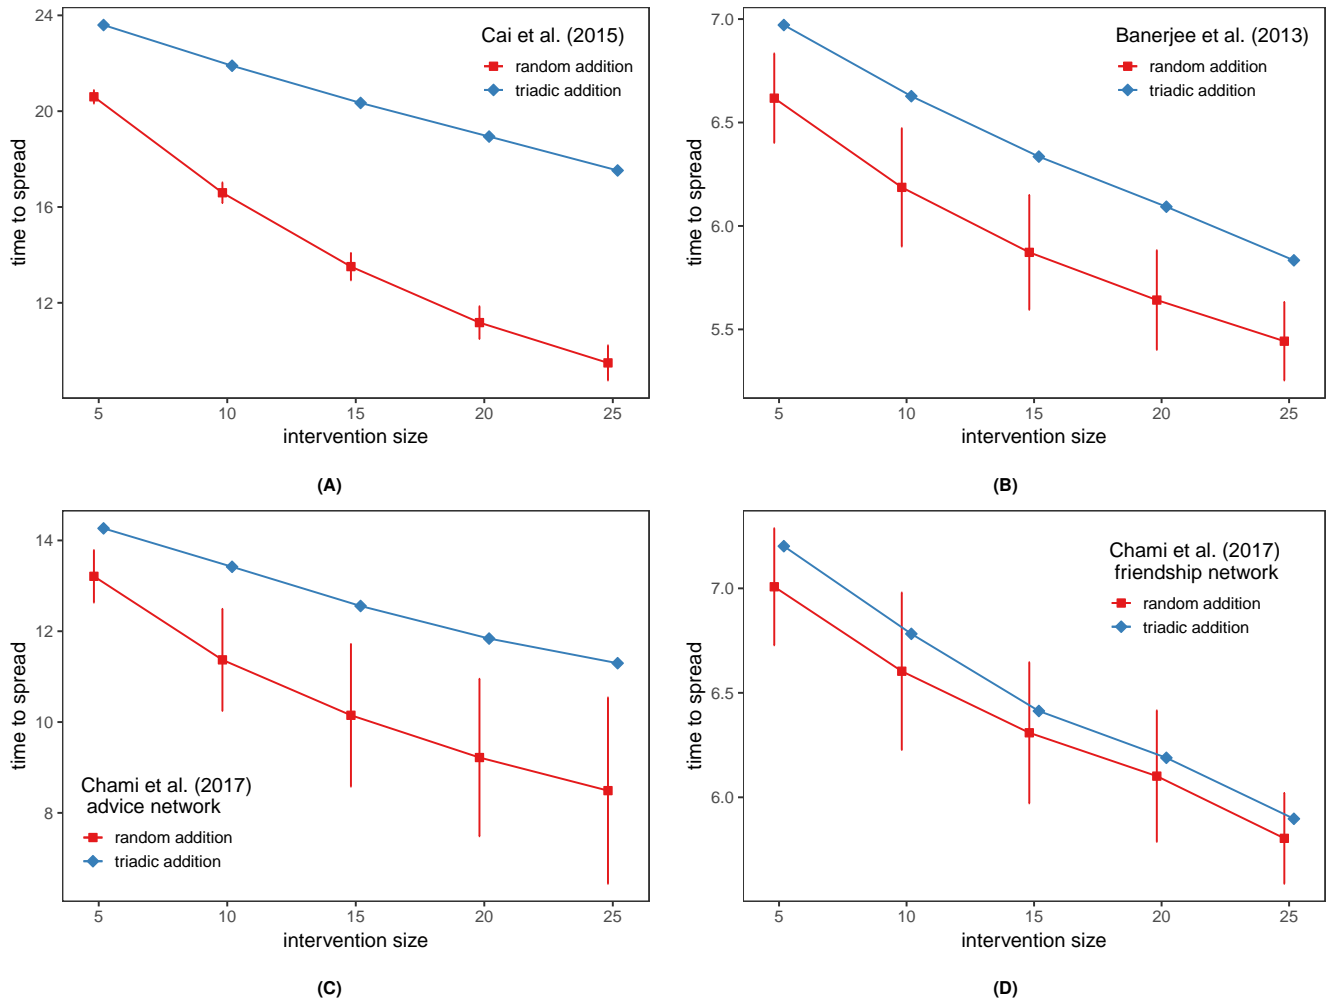

**Fig. S9.** We plot the mean time to spread in four sets of empirical networks with added triad-closing or random ties. The x-axis indicates the number of added ties (intervention size) as percent of edges in the original networks. Each point averages over all networks in that set. Error bars are 95% confidence intervals for the difference from the spread times over the networks with added triad-closing ties. We compute the confidence intervals by treating each network as a single observation.

## References

1. Aral S, Muchnik L, Sundararajan A (2009) Distinguishing influence-based contagion from homophily-driven diffusion in dynamic networks. *Proceedings of the National Academy of Sciences* 106(51):21544–21549.
2. Bakshy E, Rosenn I, Marlow C, Adamic L (2012) The role of social networks in information diffusion in *Proceedings of the 21st international conference on World Wide Web*. (ACM), pp. 519–528.
3. Centola D (2010) The spread of behavior in an online social network experiment. *science* 329(5996):1194–1197.
4. Mørsted B, Sapiezynski P, Ferrara E, Lehmann S (2017) Evidence of complex contagion of information in social media: An experiment using twitter bots. *PloS one* 12(9):e0184148.
5. Ugander J, Backstrom L, Marlow C, Kleinberg J (2012) Structural diversity in social contagion. *Proceedings of the National Academy of Sciences* 109(16):5962–5966.
6. Doerr B (2011) Analyzing randomized search heuristics: Tools from probability theory in *Theory of Randomized Search Heuristics: Foundations and Recent Developments*. (World Scientific), pp. 1–20.
7. Janson S (2018) Tail bounds for sums of geometric and exponential variables. *Statistics & Probability letters* 135:1–6.
8. Cai J, De Janvry A, Sadoulet E (2015) Social networks and the decision to insure. *American Economic Journal: Applied Economics* 7(2):81–108.
9. Chami GF, Ahnert SE, Kabatereine NB, Tukahebwa EM (2017) Social network fragmentation and community health. *Proceedings of the National Academy of Sciences* 114(36):E7425–E7431.
10. Banerjee A, Chandrasekhar AG, Duflo E, Jackson MO (2013) The diffusion of microfinance. *Science* 341(6144):1236498.
11. Traud AL, Mucha PJ, Porter MA (2012) Social structure of facebook networks. *Physica A: Statistical Mechanics and its Applications* 391(16):4165–4180.
